# Supplementary material for: Information Source Finding in Networks: Querying with Budgets
Source: arXiv:2009.00795 source file (2020-10-22)
Supplement: Supplementary file 1 [file appendix.tex]

\section*{Appendix: Proof of Results}
In this section, we will provide the
proofs of Proposition~\ref{pro:subOPT} and Theorems.
\label{sec:proof}

\subsection{Proof of Proposition~\ref{pro:subOPT}}
First, note that the {\bf SUB-OPT-NA} is represented by
\begin{align}
  \label{eq:trade1}
&\max_{v \in C_r} \bprob{G_N,A_{r}(p,q) | v=v_1} \cr
& =  \max_{v \in C_r} \bprob{G_N,A_{r}(p,q)|v=v_1, v_1 \in C_r} \times \prob{v_1 \in
  C_r}.
\end{align}
We will prove that the RC-based algorithm maximizes for both probabilities
in \eqref{eq:trade1}. First, we consider the second probability.
To see this, suppose $V_{K/r} :=\{v(1),\ldots, v(K/r)\}$ is the
set which contains $K$-largest rumor centrality nodes and let $P(v(i)
=v_1) ~(1\leq i \leq K/r)$ be the source detection probability \ie, the
probability that the $i$-th largest rumor centrality node is the rumor
source. Let $S$ be a set of infected nodes with $|S|=K$ then our
objective is to find
\begin{equation*}
\begin{aligned}
S^* =\arg\max_{S\subset G_N, |S|=K/r}\mathbb{P}(v_1 \in S |G_N).
\end{aligned}
\end{equation*}
Since the probability $P(v_1 \in S |G_N)$ is given by
\begin{align*}
\mathbb{P}(v_1 \in S |G_N)&=\sum_{v \in
  S}\mathbb{P}(v=v_1|G_N)\\ &=\sum_{v \in S}\frac{\mathbb{P}(v=v_1 ,
  G_N)}{\mathbb{P}(G_N)}\\ &=\sum_{v \in S}\frac{P(v=v_1 ,
  G_N)}{\mathbb{P}(v=v_1)}\frac{\mathbb{P}(v=v_1)}{\mathbb{P}(G_N)}\\ &=\sum_{v
  \in
  S}\mathbb{P}(G_N|v=v_1)\frac{\mathbb{P}(v=v_1)}{\mathbb{P}(G_N)},\\
\end{align*}
where $P(G_N)=\sum_{v \in G_N}P(G_N |v)P(v=v_1)$ is independent how
choose the set $S$ and $P(v=v_1)$ is same for all $v \in G_N $. Hence,
we have
\begin{equation*}
\begin{aligned}
\mathbb{P}(v_1 \in S |G_N) &\propto \sum_{v \in
  S}\mathbb{P}(G_N|v=v_1)\propto \sum_{v \in S}R(v, V_N).
\end{aligned}
\end{equation*}
Therefore, the probability $\mathbb{P}(v_1 \in S |G_N)$ is maximum
when $S=V_{K/r}$. Next, we consider the first probability in \eqref{eq:trade1}.
Indeed, this term is also decomposed by
\begin{equation}  \label{eq:trade2}
\begin{aligned}
&\bprob{G_N,A_{r}(p,q)|v=v_1, v_1 \in C_r}\\
&= \bprob{G_N|v=v_1, v_1 \in C_r}\bprob{A_{r}(p,q)|v=v_1, v_1 \in C_r}.
\end{aligned}
\end{equation}
Then, one can check that the first probability in \eqref{eq:trade2} is maximized
when the $C_r =V_{K/r}$. Furthermore, the second probability is independent of
set $C_r$ because the querying data is independent to this set. Hence, we obtain
$C_{r}^* = V_{K/r}$ and this completes the proof of
Proposition~\ref{pro:subOPT}.

\subsection{Proof of Theorem~\ref{theorem:lower}}
First, for a given $r,$ we introduce the notation $V_l,$ which is
equivalent to $C_r,$ where the hop distance $l=\frac{\log\left(\frac{K(d-2)}{rd}+2\right)}{\log(d-1)}$.
 Also for notational simplicity, we simply use $
\prob{\hat{v}=v_{1}}$ to refer to $\lim_{N \to \infty }\prob{\hat{v}(G_N,r)=v_{1}}$
for any estimator given the snapshot $G_N$ and redundancy parameter $r$ in the proof section.
Then, the detection probability is expressed as the product of the two
terms:
    \begin{align}
      \label{eqn:detect0}
      \prob{\hat{v} = v_{1}} &=   \prob{v_1 \in  V_{l}}\times  \prob{\hat{v}=v_1|v_1 \in V_{l}},
    \end{align}
where the first one is the probability that the source is in the $l$-hop based candidate set $V_l$
and the second term is the probability that the estimated node is exactly the source in the candidate set for
any learning algorithm under the algorithm class $\mathcal{C}(l,r)$.
We first obtain the upper bound of probability of first term in \eqref{eqn:detect0}
in the following lemma.

\smallskip
\begin{lemma}\label{lem:multihop_upper}
For $d$-regular trees,
\begin{equation}
\prob{v_1 \in V_{l}} \leq 1-c\cdot e^{-l\log l},
\label{eqn:multihop_upper}
\end{equation}
where $c = 4d/3(d-2)$.
\end{lemma}
\smallskip

\begin{proof}
To obtain the results. To do this,
we decompose the event $\{d(v_1,v_{RC})=i\}$ into sub-events where $v_{RC}$ has been
infected in different moment so that
\begin{equation*}
\prob{d(v_1,v_{RC}) = l} = \sum_{k=l+1}^\infty \prob{v_{RC} = v_k} \prob{d(v_1,v_k) = l},
\end{equation*}
where $v_k$ is the $k$-th infected node. The summation of series starts from $k = i+1$, since the node infected
after $(l+1)$-th order cannot be placed within distance $l$ from $v_1$.
We now obtain $\prob{d(v_1,v_k)=l}$ as follows.

\smallskip
\begin{proposition}
$\prob{d(v_1,v_k) = l}$ is given by
\begin{equation}
\prob{d(v_1,v_k) = l} = \frac{G(k-2,k-l-1)}{\prod_{j=1}^{k-1}(2 + j(d-2))} d (d-1)^{l-1},
\label{eqn:interactive_multihop}
\end{equation}
here $ G(a,b) \triangleq \sum_{\mathcal{I} \subset \{1, \cdots, a\}, |\mathcal{I}| = b} \left(\prod_{l \in \mathcal{I}} \{1 + l(d-2)\}\right). $
where $\mathcal{I}$ is any subset of $\{1, \cdots, a\}$ with cardinality $|\mathcal{I}| = b$.
\label{pro:interactive_multihop}
\end{proposition}
\smallskip
We will provide the proof of Proposition~\ref{pro:interactive_multihop} in later.
From this result, we have
\begin{equation*}
 \begin{aligned}
\prob{&d(v_1,v_k) = l} = \frac{G(k-2,k-l-1)}{\prod_{j=1}^{k-1}(2 + j(d-2))} d (d-1)^{l-1}\\
&\leq \sum_{\mathcal{I} \subset \{1, \cdots, k\}, |\mathcal{I}| = k-l-1}\frac{d (d-1)^{l-1}}{(k-1)d}\left(\frac{d-1}{d}\right)^{k}\\
&\stackrel{(a)}{=}\binom{k}{k-l-1}\frac{(d-1)^{l-1}}{(k-1)}\left(\frac{d-1}{d}\right)^{k}\\
&\leq\frac{(k-l)^{l-1}d^{l}}{k}\left(\frac{d-1}{d}\right)^{k},\\
  \end{aligned}
\end{equation*}
where $(a)$ follows from the fact that the cardinality of summation is same for the number of possible ways of $k-l-1$ among $k-2$.
It is shown that \cite{shah2012}
$\prob{v_{RC} = v_k} \leq \frac{1}{k}.$
By using these lower bound, we have
 \begin{align*}
\prob{&d(v_1,v_{RC}) = l} = \sum_{k=i+1}^\infty \text{Pr}(v_{RC} = v_k) \text{Pr}(d(v_1,v_k) = l)\\
&\leq \sum_{k=l+1}^\infty\frac{(k-l)^{l-1}d^{l}}{k}\left(\frac{d-1}{d}\right)^{k}\frac{1}{k}\\
&= \sum_{k=l+1}^\infty\frac{(k-l)^{l-1}d^{l}}{k^2}\left(\frac{d-1}{d}\right)^{k}\\
&\leq \left(\frac{d-2}{d-1}\right)^{l-1}\sum_{k=l+1}^\infty e^{-k/4}\leq 1- \left(\frac{d-1}{d}\right)^{l} e^{- \log l}.
 \end{align*}
Then, we obtain the probability $\prob{v_1 \in V_{l}}=\sum_{i=1}^{l}\prob{d(v_1,v_{RC}) = l} \leq 1-c\cdot e^{-l\log l}$
where $c = 4d/3(d-1)$ and this completes the proof of Lemma~\ref{lem:multihop_upper}.
\end{proof}
\smallskip

We will closely look at the case of each $l$, to derive the
probability that the rumor center $v_{RC}$ is exactly $l$-hop distant
from the rumor source $v_1$. Let $\delta_1$ be the error for the $\prob{v_1 \notin V_{l}}$ then
it is lower bounded by $\delta_1 \geq c\cdot e^{-l\log l}$.

To obtain the second term in \eqref{eqn:detect0}, we use the information theoretical techniques
for the direct graph inferring in \cite{Sujay2012} with partial observation because, if the rumor spread from the source
we can obtain a direct tree where all direction of edges are outgoing from the source. By asking the id/dir question,
we can infer the revered direct tree where direction of all edges are forward to the source and in our querying model,
there may be no direction answer which gives partial observation. From the assumption
of independent answers of queries, we see that the snapshot from one querying process is equivalent to the
snapshot of diffusion from the source under the Independent Cascade (IC) diffusion model.
By using these fact and the result of graph learning from the epidemic cascades in \cite{Sujay2012}, we have the following lemma.

\smallskip
\begin{lemma}\label{lem:information}
For any graph estimator to have a probability of error of $\delta_2$, it needs $r$ queries to the candidate
set $V_l$ with $|V_l|=n$ that satisfies
\begin{equation}\label{eqn:information1}
r\geq \frac{(1-\delta_2)H(T) (n-1)\log \frac{n}{2}}{n((1-H(p))+p (1-p)(\log_2 d-H(q)))},
\end{equation}
where $H(T)$ is the entropy of infection time vector and $H(p)=p \log p + (1-p)\log (1-p)$ and $H(q)= q \log q + (1-q)\log \frac{1-q}{d-1} $, respectively.
\end{lemma}
\smallskip

\begin{proof}
Let $G$ be the direct tree where all direction of edges are forward to the source and let
$\hat{G}$ be an estimator of $G$ by querying process with untruthful answers.
Assume that there are $k$ observed direction answer with
truthful probability $q>1/d$ by one id/dir question, the detection of direct tree is given by
 \begin{align*}
\prob{G=\hat{G}}=\sum_{k=0}^{n-1}\prob{G=\hat{G}||Z_d|=k} \prob{|Z_d|=k},
 \end{align*}
where $Z_d$ is the set of obtained direction answer.
Let $Y_i$ be the random variable that represents the infection order for a node $i$ with probability
$q>1/d$, then from similar technics of information theoretic bound in \cite{Sujay2012}, we have
 \begin{align*}
\prob{G=\hat{G}||Z_d|=k} \leq \frac{k (\log_2 d -H(Y_i))}{(n-1)d \log (n/2)},
 \end{align*}
where $H(Y_i)$ is the entropy of $Y_i$ and we use the fact that we are interest in exact recovery \ie, $B(G^{'})=G^{'}$ hence
we have $|B(G^{'})|=1.$ Further, it is easy to see that $|\mathcal{G}|\geq (n-1)\log (n/2)$ from the constructed
direct tree using the querying process. The term $H(D_i)$ is the entropy of the sample
data of queried node $i$. From the Bernoulli distribution for the identity question with $p$, we have
$\prob{|Z_d|=k} \leq \binom{n}{k}p^k (1-p)^{n-k}.$ Hence, we obtain
 \begin{align*}
\prob{G=\hat{G}}&=\sum_{k=0}^{n-1}\prob{G=\hat{G}||Z_d|=k} \prob{|Z_d|=k}\cr
&\leq \sum_{k=0}^{n-1} \frac{ k(\log_2 d -H(Y_i))}{(n-1)d \log (n/2)}\binom{n}{k}p^k (1-p)^{n-k}\cr
&=\sum_{k=0}^{n}\binom{n}{k}k p^k (1-p)^{n-k} \frac{ (\log_2 d -H(Y_i))}{(n-1)d \log (n/2)}\cr
&= \frac{ np(\log_2 d -H(Y_i))}{(n-1)d \log (n/2)}.
 \end{align*}
Consider the $r$ times id/direction queries and
\begin{align*}
\sum_{i \in V_l}& H(D_i) \stackrel{(a)}{\leq} \sum_{i \in V_l} H(T_i)\sum_{i \in V_l} (1-H(X_i, Y_i))\cr
&\stackrel{(b)}{\leq}H(T)^{-1}n ((1-H(p))+p(1-p) (\log_2 d -H(q))),
\end{align*}
where $H(p):= p\log p + (1-p)\log(1-p)$ and $H(q):=  q\log q + (1-q) \log \frac{1-q}{d-1}$, respectively.
The inequality $(a)$ follows from the sub-additivity of entropy and $(b)$ is from the fact that two random
variable $X_i$ and $Y_i$ are independent.
Then, we have
\begin{align*}
\prob{G=\hat{G}}&\leq \frac{rnd(1-H(p)+p(1-p)(\log_2 d -H(q))}{H(T)(n-1)d \log (n/2)}.
\end{align*}
By setting the right term less than $1-\delta_2,$ we obtain the result and this completes the proof of Lemma~\ref{lem:information}.

\end{proof}
\smallskip

From the disjoint of two error event and by setting $\delta_1 = \delta_2 =\delta /2$ with $l=\log\left(\frac{K(d-2)}{rd}+2\right)/\log(d-1)$, we have
  \begin{align*}
     \prob{&\hat{v} \neq v_{1}} \geq c\cdot e^{-\frac{\log\left(\frac{K}{r}\right)}{\log(d-1)}\log \frac{\log\left(\frac{K}{r}\right)}{\log(d-1)}} \cr
     & + 1- \frac{K((1-H(p))+p (1-p)(\log_2 d-H(q)))}{H(T)(\frac{K}{r}-1)\log \frac{K}{2r}}\geq \delta.
    \end{align*}
From the fact that $\lambda =1$ in our setting and Lemma 2 in \cite{Sujay2012}, we obtain $H(T)\leq K/r $ and by differentiation of above lower bound with respect to $r$, we obtain
$r^*= \left \lfloor 1+\frac{4 (1-p)\{7H(p)+H(q)\}\log K}{3e\log(d-1)}\right\rfloor$ where
the derivation is given in later.
Since if we use the $r^*$, it gives the upper bound of detection probability hence,
we put it to the obtained upper-bound which is expressed as a
function of $K,$ as follows:
\begin{align}
  \label{eq:kkk1}
  &\prob{\hat{v} \neq v_{1}}  \cr
  & \geq  \frac{1}{2}\ e^{-h_1 (T,p,q) \log K\log (\log K)}+\frac{c}{4} e^{- 2 h_1 (T,p,q)\log K\log (\log K)}\cr
&   \geq  C_d e^{-h_1 (T,p,q)\log K \log (\log K)},
\end{align}
where $C_d=(c+3)/4$ and $h_1 (T,p,q)= H(T)^{-1}(1-H(p))+p(1-p)(\log_2 d-H(q))$. If we set $\delta \leq C_d e^{-h_1 (T,p,q)\log K\log (\log K)},$ we find the value of $K$ such that its assignment to
\eqref{eq:kkk1} produces the error probability $\delta,$ and we finally obtain the
desired lower-bound of $K$ as in Theorem~\ref{theorem:lower}.

\subsection{Proof of Theorem~\ref{theorem:noninteractive}}

We first provide the lower bound of detection probability of {\bf
  MVNA}$(r)$ for a given $K$ and $r$ in the following lemma. \note{How about presenting the results of detection probabilities in the main result section?}

\smallskip
\begin{lemma}
  \label{lem:simple_prob}
  For $d$-regular trees ($d\geq 3$), a given budget
  $K,$ our estimator $\hat{v}$ from {\bf MVNA}$(r)$ has the
  following lower-bound of the detection probability:
\begin{multline}
  \label{eqn:detect}
\prob{\hat{v}=v_{1}}\geq 1-c\left(\frac{r+p+q}{r+2}\right)^3\cdot
  \exp\Bigg( \frac{-h_d
  (K,r)w_d (p,q)}{2}\Bigg),
\end{multline}
where $c = 7(d+1)/d$ and $w_d (p,q)=\frac{1}{2}(4(p-1/2)^2+(d/(d-1))^3 (q-1/d)^3)$.
The term $h_d (K,r)$ is given by
$$h_d (K,r):=\frac{\log\left(\frac{K}{r}\right)}{\log(d-1)}\log\left(
\frac{\log\left(\frac{K}{r}\right)}{\log(d-1)}\right).$$
\end{lemma}
\smallskip

\begin{proof}
Under the {\bf MVNA}$(r)$, the detection probability is expressed as the product of the three
terms:
    \begin{align}
      \label{eqn:detection}
      \prob{\hat{v} = v_{1}} &=   \prob{v_1 \in  V_{l}}\times  \prob{\hat{v}=v_1|v_1 \in V_{l}} \cr
                               & = \prob{v_1 \in  V_{l}} \times \prob{v_1
                                 \in \hat{V}|v_1 \in V_{l}}   \cr
                               &  \times \prob{v_1 =v_{LRC}|v_1 \in \hat{V}},
    \end{align}
where $\hat{V}:=S_I \cap S_D$ if it is not empty or $\hat{V}:=S_I \cup S_D$, otherwise. This is the filtered candidate set in {\bf
  MVNA}$(r)$ and  $v_{LRC}$ is the node in $\hat{V}$ that has the
highest rumor centrality \ie, likelihood, where $LRC$ means the local rumor center.
We will drive the lower bounds of the first, second, and the third terms
of RHS of \eqref{eqn:detection}.
The first term of RHS of \eqref{eqn:detection} is bounded by
\begin{align}
  \label{eq:first}
  \prob{v_1 \in V_{l}} \geq 1-c\cdot e^{-(l/2)\log l},
\end{align}
where the constant $c = 7(d+1)/d$ from Corollary 2 of \cite{Khim14}.
Let $S_N$ be the set of revealed nodes itself as the rumor source and let $S_I$ be the set of nodes which minimizing the errors.
If the true source is in $V_{l},$ then the probability that it is most indicated node for
a given budget $K$ with the repetition count $r$ and truth probability $p>1/2$ and $q>1/d$ is given by
    \begin{align}\label{eqn:d}
      \prob{v_1 &=v_{LRC}|v_1 \in \hat{V}}\cr
     & =\prob{v_1= \arg\max_{v\in S_I\cap S_D}R(v,G_{N})|K,p,q}.
    \end{align}
To obtain this, we consider that
if $p>1/2$,
 the probability $v_1 \in S_I$ by the majority voting, because the selected node can be designation again
in the algorithm. We let total number of queries by $r\geq1$, we let $W=\sum_{i=1}^{r}X_i (v_1)$ for the source node $v_1$, then
the probability that true source is in the filtration set $S_I$ is given by
\begin{equation*}
    \begin{aligned}
     \prob{W\geq r/2}&=\sum_{j=0}^{\lfloor r/2\rfloor}\binom{ r}{j}(1-p)^{j}p^{r-j}\\
    \end{aligned}
  \end{equation*}
Then, from this relation, we have the following lemmas
whose proofs are will be provided in \cite{Choi17}:
\begin{lemma}(\cite{Choi17})
When $p>1/2,$
\begin{eqnarray*}
\prob{v_1 \in S_I|v_1 \in V_{l}}  & \geq &p+(1-p)(1-e^{-p^{2}\log r}).
\end{eqnarray*}
\label{lem:majority}
\end{lemma}
This result shows that the filtration step for the identity questions to include the
source in $S_I$. Next, we will provide the probability that the source is in the filtration
set for the direction question $S_D$ as follows. Next, we will obtain the filtered direction answer as follows.
First, consider the total number of direction queries $N_d$ is a random variable
with the distribution is Binomial:
\begin{align*}
P(N_d = k)=\begin{cases}
\binom{r}{k}p^{r -k}(1-p)^{k}&\mbox{if}~v=v_1\\
\binom{r}{k}(1-p)^{r -k}p^{k}&\mbox{if}~v \neq v_1,
\end{cases}
\end{align*}
where $k$ is less than the total repetition count $r$. Using this fact, we obtain the following result
that the source is also in the filtration set $S_D$ for the direction question.
\smallskip

\begin{lemma}
When $p>1/2$ and $q>1/d$,
\begin{eqnarray*}
\prob{v_1 \in S_D|v_1 \in V_{l}}  & \geq & 1- e^{-\frac{rp(d-1)(q-1/d)^2}{3d}}.
\end{eqnarray*}
\label{lem:consistence}
\end{lemma}
\smallskip

\begin{proof}
We first consider the following result which is the lower bound of probability
of determine the true parent among the direction answers. To see this, we let
$Y^{1}_i(v)$ be the random variable which takes $+1$ for the $i$-th query
when the true parent node is designated by the respondent $v$ with probability $q$ and let
$Y^{j}_i(v)$ be the random variable which takes $+1$ for the $i$-th query
when one of other neighbor nodes $2\leq j\leq d$ is designated by $v$ with probability
$(1-q)/(d-1)$. Let $Z_j (v):=\sum_{i=1}^{k}Y^{j}_i (v)$ be the total number of designations by the node
$v$ for the $j$-the neighbor $(1\leq j \leq d)$. Then, we need to find $\prob{Z_1 (v) > Z_j
(v),~ \forall j}$ which is the probability that the true parent is the node with maximum designations
by respondent $v$. Then, from Hoeffding bound, we obtain the following lemma.

\smallskip
\begin{lemma}
Suppose there are $k\leq r$ answers for the direction questions with $q>1/d$ then
\begin{align*}
\prob{Z_1 (v) > Z_j
(v),~ \forall j}\geq 1- e^{-\frac{k(d-1)(q-1/d)^2}{3d(1-q)}}.
\end{align*}
\label{lem:major}
\vspace{-0.5cm}
\end{lemma}
\smallskip

\begin{proof}
For a given $r$, we have
    \begin{align*}
     \prob{Z_1 (v) &\geq Z_j (v),~ \forall j}=\bprob{\sum_{i=1}^{k}Y^{1}_i (v) \geq
      \sum_{i=1}^{k}Y^{j}_i (v),~\forall j\neq 1}\\ &\geq
      \bprob{\sum_{i=1}^{k}Y^{1}_i (v) \geq \mu_1
      +\varepsilon_1}\\ &\qquad +\left(1-
      \bprob{\sum_{i=1}^{k}Y^{j}_i (v) \geq \mu_1+\varepsilon_1
      ~\forall j\neq 1}\right)\\ &\stackrel{(a)}{\geq} 1-
      \sum_{j=2}^{d}\prob{\sum_{i=1}^{k}Y^{j}_i (v) \geq
      \mu_j+\varepsilon_j }\\ &\stackrel{(b)}{\geq}
      1-(d-1)e^{-\frac{\varepsilon^2 \mu_j}{ 3}}\geq 1-
      e^{-\frac{\varepsilon^2(d-1)k(q-1/d)^2}{3dq(1-q)}},
    \end{align*}
where $\mu_1=\mathbb{E}[Z_j (v) =\sum_{i=1}^{k}Y^{j}_i (v)]=kq$ and
$\mu_j=\mathbb{E}[Z_j (v) =\sum_{i=1}^{k}Y^{j}_i
  (v)]=k(1-q)/(d-1)$. The inequality $(a)$ comes from the fact that
$\mu_1 \geq \mu_j$ for $2\leq j \leq d$ and the union
bound of probability. From Chernoff-Hoeffding bound of $Y^{j}_i (v)$,
we obtain the inequality $(b)$ by using $\varepsilon_j =\varepsilon \mu_j$.
If we set $\varepsilon = q^{1/2}$ then we obtain
$\hat{q}\geq 1-e^{-\frac{k(d-1)(q-1/d)^2}{3d(1-q)}}$ which completes the proof
of Lemma~ \ref{lem:major}.
\end{proof}

Now, we let $Err(v)$ be the set of inconsistence edges in the snapshot of direction question from a node $v$, and $|Err(v)|$ be the total number of such edges. Then, we have the following lemma.

\smallskip
\begin{lemma}
Suppose $v_1 \in V_l$ and $|Err(v_1)|=s$ for $0\leq s \leq |V_l|$ with . Then
\begin{equation}\label{eqn:d2}
    \begin{aligned}
      \prob{v_1 \in S_D ||Err(v_1)|=s}\geq \frac{|V_l|-s}{|V_l|},
    \end{aligned}
  \end{equation}
  where $|V_l|=\frac{d(d-1)^l -2}{d-2}$.
\label{lem:intersection}
\end{lemma}
\smallskip

\begin{proof}
Since we have
\begin{equation}\label{eqn:2}
    \begin{aligned}
      \prob{v_1 \in S_I |&|Err(v_1)|=s}\\
      &=\prob{\text{$|Err(v)|\geq s$ for all node $v \in V_{l}$}}\\
      &=1-\prob{\text{$\exists ~v \in V_{l}$ s.t. $|Err(v)|< s$ }})\\
      &\stackrel{(a)}{\geq} 1-\frac{s}{|V_l|},
    \end{aligned}
  \end{equation}
where $(a)$ is from the fact that for the node $d(v):=d(v,v_1)$,
    \begin{align*}
      \prob{&\text{$\exists ~v \in V_{l}$ s.t. $|Err(v)|< s$ }||Err(v_1)|=s}\\
      &\stackrel{(a)}{=}\sum_{v \in V_l}\left(\frac{d(v)}{|V_l|}\sum_{j=\lfloor d(v)/2 \rfloor}^{d(v)}s\binom{d(v)}{j}q^{d(v)-j}(1-q)^{j}\right)\\
      &\leq \frac{2l}{|V_l|}\sum_{j=l}^{2l}\frac{s}{2l}\binom{2l}{j}q^{2l-j}(1-q)^{j}\\
       &= \frac{1}{|V_l|}\sum_{j=l}^{2l}s\binom{2l}{j}q^{2l-j}(1-q)^{j}\\
        &\stackrel{(b)}{\leq} \frac{1}{|V_l|}\left[\sum_{j=1 }^{|V_l|}s\binom{|V_l|}{j}q^{|V_l|-j}(1-q)^{j}\right]= \frac{s}{|V_l|},
    \end{align*}
where $(a)$ is from the fact that for a fixed node $v \in V_l$, the probability of selecting the edges between of them is
$d(v)/|V_l|$ with the union bound and the second therm is the probability that some of them are changed which is a binomial distribution.
The inequality $(b)$ by letting $2l <|V_l|$.
%where $(a)$ is the edges on the path between $v$ and $v_1$ is changed.
Hence, we have the result of \eqref{eqn:d2}
and this completes the proof of Lemma~\ref{lem:intersection}.
\end{proof}
Using above two lemmas and from the fact that there are $np$ nodes that are not determined as the source in expectation by the Binomial distribution, we finally obtain the result of Lemma \ref{lem:consistence} and this completes the proof.
\end{proof}

We can use this result directly in our case because the identity question is queried by
the number of $r$ that is the total query to a node. The number of direction questions may be different.
By considering the two results in the above, we have the following lemma.

\smallskip
\begin{lemma}
For given repetition count $r$,
\begin{equation}\label{eqn:d1}
    \begin{aligned}
      P(v_1 \in S_I \cap S_D|v_1 \in V_l) \geq 1-2e^{-f(p,q) 2r\log r}
    \end{aligned}
  \end{equation}
where $f (p,q)=3(p-1/2)^2 + \frac{d-1}{3d} p(1-p)(q-1/d)^2$.
\label{lem:finalfil}
\end{lemma}
\smallskip

\begin{proof}
From that fact that the events of $v_1 \in S_I$ and $v_1 \in S_D$ are independent for given $K,p,q$ since
first one is the results of source itself and the second one is the result from the other nodes. Then, we have
\begin{equation*}
    \begin{aligned}
         \prob{v_1 &\in S_I \cap S_D |v_1 \in V_l}\\
         &=\prob{v_1 \in S_I|v_1 \in V_l)P(v_1 \in  S_D|v_1 \in V_l}\\
         & \geq \left(p+(1-p)(1-e^{-p^{2}\log r})\right)\left(1- e^{-\frac{r(d-1)(q-1/d)^2}{3d}}\right)\\
          & \stackrel{(a)}{\geq} \left(1-e^{-3(p-1/2)^{2}\log r}\right)\left(1- e^{-\frac{r(d-1)(q-1/d)^2}{3d}}\right)\\
         & \stackrel{(b)}{\geq} 1-2e^{-f(p,q) 2r\log r},
    \end{aligned}
  \end{equation*}
 where $(a)$ is from the fact that $p>1/2$ and $(b)$ can be obtained by simple algebra with $f_1 (p,q)=c_1 (p-1/2)^2 + c_2 p(1-p)(q-1/d)^2 $ for some constants $c_1 =3$ and $c_2 = (d-1)/3d$. This completes the proof of Lemma \ref{lem:finalfil}.
\end{proof}

Next, we consider the following lemma which indicates the lower bound of detection probability
among the final candidate set.

\smallskip
\begin{lemma} \label{lem:filtration}
  When $d\geq3$, $p>1/2$ and $q>1/d$,
  \begin{eqnarray*}
    \prob{v_1 =v_{LRC}|v_1 \in S_I \cap S_D}  & \geq & 1-e^{-f(p,q) r\log r}.
  \end{eqnarray*}
\end{lemma}
\smallskip

\begin{proof}
To prove this, we let $X(n,\hat{p},\hat{q})$ be the random variable that
indicates the number of nodes which reveals itself as the rumor source
among $n$ nodes. Then, from \cite{dong2013}, we have that if $X(n,\hat{p},\hat{q})=k$
then
\begin{equation*}
    \begin{aligned}
      \varphi_{d}(K,r)\geq 1-\frac{2(k-1)}{k}\left(1-I_{1/2}
      \left( \frac{1}{d-2}, \frac{d-1}{d-2} \right)\right),
    \end{aligned}
  \end{equation*}
  where $I_\alpha (a, b)$ is a regularized incomplete Beta function:
\begin{equation*}
I_\alpha (a, b) = \frac{\Gamma(a+b)}{\Gamma(a)\Gamma(b)} \int_0^\alpha t^{a-1} (1-t)^{b-1}dt,
\end{equation*}
where $\Gamma(\cdot)$ is the standard Gamma function
Clearly, the right term is a decreasing function with respect to $k$
and it has the minimum at $k$ is infinity as $1/2$ and maximum at
$k=1$ as one.
From the previous result, we know that if the
repetition count $r$ increase then $\hat{p}$ goes to one. Based on this, we
will show that if $p>1/2$ and $r\geq 1$ then
$\prob{X(n,\hat{p})> 1}\leq e^{-p^{2}r\log r}$
where $n=\frac{d(d-1)^l -2}{d-2}$. To do this, we let $Y$ be the
Bernoulli random variable which takes value $+1$ (\ie tell itself as the
source node $i=j$ ) w.p. $\hat{p}$ for the source node and takes $0,$
otherwise. Let $X=\sum_{i=1}^{n-1}X_i$ be the sum of Bernoulli random
variables where $X_i$ takes 1 w.p. $1-\hat{p}$ and 0, otherwise. Then,
we will obtain that $\mathbb{P}(X+Y\geq 2)\leq e^{-f (p,q)^{2}r\log r}$. To
see this, it is sufficient to show that $\mathbb{P}(X\geq 1)\leq
e^{-p^{2}r\log r}$. Let $E[X]=\mu=(n-1)(1-\hat{p})$ then from the
Chernoff bound, we have
\begin{equation}\label{eqn:Chernoff}
    \begin{aligned}
\bprob{\sum_{i=1}^{n-1}X_i \geq \mu+\varepsilon}\leq
e^{-\varepsilon^2 \mu}.
    \end{aligned}
  \end{equation}
From Lemma~\ref{lem:majority}, one can check that $\hat{p}\geq
p+(1-p)(1-e^{-p^{2}\log r})< 1-\frac{1}{n-1}$ which implies
$\mu=(n-1)(1-\hat{p})<1$.  Then, by using this and
\eqref{eqn:Chernoff}, we obtain $\mathbb{P}(X\geq 1)\leq
e^{-p^{2}r\log r}$.  Finally, from these results, the probability
$\varphi_{d}(n,\hat{p})$ is given by
\begin{equation}
    \begin{aligned}
      \varphi_{d}(K,r)&=\sum_{k=1}^{n}\mathbb{P}(\hat{v}=
      v_{1}|X(n,\hat{p})=k)\prob{X(n,\hat{p})=k}\\ &=
      \mathbb{P}(\hat{v}=
      v_{1}|X(n,\hat{p})=k)\prob{X(n,\hat{p})=k} \\ & \quad
      +\sum_{k=2}^{n}\prob{\hat{v}=
      v_{1}|X(n,\hat{p})=k}\prob{X(n,\hat{p})=k}\\ &\geq 1-
      e^{-f (p,q)^{2}r\log r},\\
    \end{aligned}
  \end{equation}
which completes the proof of Lemma \ref{lem:filtration}.
\end{proof}

Merging these lower-bound with the lower-bound in
\eqref{eq:first} where we plug in
$l=\frac{\log\left(\frac{K(d-2)}{rd}+2\right)}{\log(d-1)},$ we finally get the lower bound of detection probability
 of {\bf MVNA}$(r)$ for a given repetition count $r$ and this completes the proof of
 Lemma~\ref{lem:simple_prob}.
\end{proof}

The second term of RHS of \eqref{eqn:detect} is the probability that the
source is in the candidate set for given $K$ and $r$. Hence, one can see
that for a fixed $K$, large $r$ leads to the decreasing detection
probability due to the smaller candidate set.  However, increasing $r$
positively affects the first term of RHS of \eqref{eqn:detect}, so that
there is a trade off in selecting a proper $r$.
By derivation of the result with respect to $r$, we first obtain $r^*$ which maximizes the detection
probability by $r^*= \left \lfloor 1+\frac{2(1-p)\{1+(1-q)^2\}\log K}{e\log(d-1)}\right\rfloor$ in {\bf MVNA}$(r^*)$
and put this into the error probability $\prob{\hat{v}\neq v_{1}}$ such as

\begin{align}
  \label{eq:ppp}
  \prob{\hat{v}&\neq v_{1}} \leq e^{-f(p,q) r\log r}+2e^{-f(p,q) 2r\log r}+c\cdot e^{- \frac{l}{2}\log l},
\end{align}
where the constant $c$ is the same as that in \eqref{eq:first}.
Now, we first put
$l=\frac{\log\left(\frac{K(d-2)}{rd}+2\right)}{\log(d-1)}$ into
\eqref{eq:ppp} and obtained the upper-bound of \eqref{eq:ppp}, expressed
as a function of $r,$ for a given $p$ and $q$ and the constant $c.$
Then, we take $r^*$ and put it to the obtained upper-bound which is expressed as a
function of $K,$ as follows:
\begin{align}
  \label{eq:kkk2}
  \prob{\hat{v} \neq v_{1}}  & \leq  3\ e^{-f(p,q) \log K\log (\log K)}+c e^{- \frac{\log K}{2}\log (\log K)}\cr
&   \leq  c_1 e^{-f (p,q)\log K \log (\log K)},
\end{align}
where $c_1=c+3$. If we set $\delta \geq c_1 e^{-f (p,q)\log K\log (\log K)},$ we find the value of $K$ such that its assignment to
\eqref{eq:kkk2} produces the error probability $\delta,$ and we get the
desired lower-bound of $K$ as in the theorem statement. This completes
the proof.

\subsection{Proof of Theorem~\ref{theorem:lowerad}}
We will show the lower bound for given $K$ and $r$ of the case $p<1$. \footnote{The result
  for $p=1$ is similar except the termination of querying process when it meets the source.}
For a given $r,$ we let $V_s$ be the set of all infected nodes from the rumor source within distance $K/r$ then we see that
the querying dynamic still becomes a directed tree construction rooted by the source $v^*$.
Then, the detection probability is expressed as the product of the two
terms:
    \begin{align}
      \label{eqn:detect01}
      \prob{\hat{v} = v_{1}} &=   \prob{v_1 \in  V_{s}}\times  \prob{\hat{v}=v_1|v_1 \in V_{s}},
    \end{align}
where the first one is the probability that the distance between source and rumor center is less than $K/r$
and the second term is the probability that the estimated node is exactly the source in the candidate set for
any learning algorithm under the algorithm class $\boldsymbol{C}(nb,r)$.
First, from Lemma~\ref{lem:multihop_upper}, we have that the probability of first term in \eqref{eqn:detect01} is
upper bounded by $1-ce^{-(K/r)\log(K/r)}$ where $c=4d/3(d-2)$ for a given budget $K$ and repetition count $r$.
We see that
the querying dynamic still becomes a directed tree construction rooted by the source $v^*$.
However, different to the NA-querying, the querying process gives direction data of a subgraph of the original direct tree
because the querier chooses a node, interactively.
For a given $r$, let $Z_{r,i}$ be the answer data of querying for a selected queried node $i$ where $1 \leq i \leq K/r.$ Then,
from the assumption of the algorithm class $\boldsymbol{C}(nb,r)$,
the joint entropy for the random answers with the infection time random vector $T$,
$(T, Z_{r,1},\ldots,Z_{r,K/r})$ is given by
 \begin{align}\label{eqn:entropy}
     H(T, Z_{r,1},&\ldots,Z_{r,K/r})=\sum_{i=1}^{K/r}H(T, Z_{r,i}|Z_{r,i-1},\ldots,Z_{r,1})\cr
     &=\sum_{i=1}^{K/r}H(T, Z_{r,i}|Z_{r,i-1})\stackrel{(a)}{=}\sum_{i=1}^{K/r}H(T, Z_{r,i}),
    \end{align}
where $(a)$ is from the fact that all data $Z_{r,i}$ are independent.
Let $G^*$ be the true directed graph and let $\hat{G}$ be be an estimated directed tree from the
sequential answers of adaptive querying $(Z_{r,1},\ldots,Z_{r,K/r})$. Then, we see that
this defines a Markov chain
$$G^* \rightarrow (T, Z_{r,1},\ldots,Z_{r,K/r}) \rightarrow \hat{G},$$
from the defined algorithm class $\boldsymbol{C}(nb,r)$. By property of the mutual information, we have
 \begin{align}\label{eqn:entropy1}
    I(G^*; &T, Z_{r,1},\ldots,Z_{r,K/r})\cr
    &\leq H(T, Z_{r,1},\ldots,Z_{r,K/r})=\sum_{i=1}^{K/r}H(T, Z_{r,i}) \cr
    &\stackrel{(a)}{=} (K/r)H(T, Z_{r,1})\cr
    &\stackrel{(b)}{\leq} (K/rH(T))[r(1-H(p))+rp(\log_2 d - H(q))]\cr
    &= K[(1-H(p))+p(\log_2 d - H(q))]:=Kh(p,q),
    \end{align}
where $(a)$ follows from the fact that the answers $Z_{r,i}$ are mutually exclusive
and $(b)$ is from the fact that $H(T, Z_{r,1})=(1-H(p)+rp(\log_2 d - H(q)))/H(T)$ since
the number of direction answers follows binomial distribution. Let $\mathcal{G}_{K/r}$ be the
set of possible directed tree in $V_s$ then we have $|\mathcal{G}_{K/r}|\leq (K/r)\log (K/2r)$.
Using the Fano's inequality on the Markov chain $G^* \rightarrow (Z_{r,1},\ldots,Z_{r,K/r}) \rightarrow \hat{G},$
we obtain
 \begin{align}\label{eqn:entropy2}
   \prob{G \neq G^*}&=\prob{\hat{v} = v_{1}|v^* \in V_s}\cr
   &\geq 1- \frac{I(G^*; Z_{r,1},\ldots,Z_{r,K/r})+h(p,q)}{H(T)\log|\mathcal{G}_{K/r}|}\cr
   & \geq 1- \frac{Kh(p,q)+h(p,q)}{\frac{KH(T)}{r}\log (\frac{K}{2r}-1)}.
    \end{align}
By solving $r$, we have if $r\leq (1-\delta) H(T)(\log K -1)/h(p,q)\log_2 d $ then, $\prob{\hat{v} = v_{1}|v^* \in V_s}\geq \delta.$
From the disjoint of two error event and by setting $\delta_1 = \delta_2 =\delta /2$ for each error, we have
  \begin{align}\label{eqn:entropy3}
     \prob{&\hat{v} \neq v_{1}} \geq c\cdot e^{-(K/r)\log(K/r)} \cr
     & + 1- \frac{Kh(p,q)+h(p,q)}{\frac{KH(T)}{r}\log (\frac{K}{2r}-1)}\geq \delta.
    \end{align}
From the fact that $\lambda =1$ in our setting and Lemma 2 in \cite{Sujay2012}, we obtain $H(T)\leq K/r $ and
by differentiation of above lower bound with respect to $r$, we obtain
$r^*= \left \lfloor 1+\frac{7 dp\{3H(p)+2dH(q)\}\log \log K}{2(d-1)}\right\rfloor$ where
the derivation is given in \cite{Jae16}.
Since if we use the $r^*$, it gives the upper bound of detection probability hence,
we put it to the obtained upper-bound which is expressed as a
function of $K,$ as follows:
\begin{align}
  \label{eq:kkk3}
  \prob{\hat{v} \neq v_{1}}  & \geq  \frac{1}{3}\ e^{-h_2(T,p,q) \log (\log K)}+\frac{c}{4} e^{- 7 h_2 (T,p,q)\log (\log K)}\cr
&   \geq  C_d e^{-h_2 (T,p,q) \log (\log K)},
\end{align}
where $C_d=2(c+3)/7$ and $h_2 (T,p,q)= H(T)^{-1}(1-H(p))+(1-p)(\log_2 d-H(q))$. If we set $\delta \leq C_d e^{-h_2 (T,p,q)\log (\log K)},$ we find the value of $K$ such that its assignment to
\eqref{eq:kkk3} produces the error probability $\delta,$ and we get the
desired lower-bound of $K$ as in the theorem statement.
Then, we finally obtain the result and this completes the proof of
Theorem~\ref{theorem:lowerad}.

\subsection{Proof of Theorem~\ref{theorem:interactive}}
We will show the lower bound of the detection
  probability for given $K$ and $r$ of the case $p<1$ \footnote{The result
  for $p=1$ is given in \cite{Choi17} hence, we omit it here.} in Lemma~\ref{lem:inter_prob}.

\smallskip
\begin{lemma}
  \label{lem:inter_prob}
  For $d$-regular trees ($d\geq 3$), a given budget
  $K,$ our estimator $\hat{v}$ from {\bf MVAD}$(r)$ has the
  detection probability lower-bounded by:
\begin{align}
  \label{eqn:detect2}
&\prob{\hat{v}=v_{1}} \cr
&\ge  1-c (g_d (r,q))^3\cdot \exp\left [-\left(p-\frac{1}{2}\right)^2\left(\frac{K}{r}\right)\log \left(\frac{K}{r}\right) \right],
\end{align}
where $g_d (r,q):= 1- e^{-\frac{r(d-1)(q-1/d)^2}{3d(1-q)}}$ and
$c=(5d+1)/d$.
\end{lemma}
\smallskip

\begin{proof}
For the {\bf MVAD}$(r)$, for a given $r,$ we introduce the notation $V_s,$
where the set of all queried nodes of the algorithm. From the initial queried node, we need the probability
that the source is in the set of queried node by some policy $P \in \mathcal{P}(v_I)$.
Then, the detection probability is also expressed by the product of the three
terms:
    \begin{align}
      \label{eqn:detection1}
      \prob{\hat{v} = v_{1}} &=   \prob{v_1 \in  V_{s}}\times  \prob{\hat{v}=v_1|v_1 \in V_{s}} \cr
                               & = \prob{v_1 \in  V_{s}} \times \prob{v_1
                                 \in \hat{V}|v_1 \in V_{s}}   \cr
                               &  \times \prob{v_1 =v_{LRC}|v_1 \in \hat{V}},
    \end{align}
where $V_s = \{v| d(v_{RC},v) \le K/r\}$ because the number of budget is $K$ and $\hat{V}=S_I \cap S_D$
if it is not empty or $\hat{V}=S_I \cup S_D$, otherwise.
From the result in Corollary 2 of \cite{Khim14}, we have $\prob{E_1}\leq c \cdot e^{- (K/r)\log K/r}$
since we use additional direction query with identity question. For the second part of probability in \eqref{eqn:detection1},
we obtain the following lemma.

\smallskip
\begin{lemma}
When $p>1/2,$
\begin{equation*}
 \begin{aligned}
\prob{v_1 &\in S_I|v_1 \in V_{s}}  \\
&\geq \left(p+(1-p)(1-e^{-p^{2}\log r})\right) \left(1-ce^{-\frac{Kp}{r}  (q-1/d)^3}\right).
   \end{aligned}
   \end{equation*}
\label{lem:idinter}
\end{lemma}
\smallskip

\begin{proof}
Let $Q_K (v)$ be the number of queries to a node $v \in V_l$ when there are $K$ queries then we have
\begin{equation*}
    \begin{aligned}
     &\prob{Q(v_1)\geq1}\\
     &=\sum_{i=1}^{l}\prob{Q(v_1)\geq1|d(v_1, v_{RC})=i}\prob{d(v_1, v_{RC})=i}.
    \end{aligned}
  \end{equation*}
where $\prob{d(v_1,v_{RC}) = i}$ is the probability that the distance from the rumor center to rumor source is $i$ and this probability become smaller if the distance between rumor source and rumor center is larger.
From this, we have the following result for the lower bound of the probability of distance between the rumor center and source.
\smallskip
\begin{lemma}
For $d$-regular trees,
\begin{equation}
\prob{d(v_1,v_{RC}) = i}\geq \left(\frac{d-1}{d}\right)^{i} e^{-(i+1)}.
\label{eqn:interactive_multihop1}
\end{equation}
\label{lem:distance1}
\end{lemma}
\smallskip

We will closely look at the case of each $i$, to derive the
probability that the rumor center $v_{RC}$ is exactly $i$-hop distant
from the rumor source $v_1$.

\begin{proof}
In this section, we will provide the proof of Lemma~\ref{lem:distance1}.
To obtain the results. To do this,
we decompose the event $\{d(v_1,v_{RC})=i\}$ into sub-events where $v_{RC}$ has been
infected in different moment so that
\begin{equation*}
\prob{d(v_1,v_{RC}) = i} = \sum_{k=i+1}^\infty \prob{v_{RC} = v_k} \prob{d(v_1,v_k) = i}.
\end{equation*}
The summation of series starts from $k = i+1$, since the node infected
after $(i+1)$-th order cannot be placed within distance $i$ from $v_1$.
We now obtain $\prob{d(v_1,v_k)=i}$ as follows.

From the results of Proposition~\ref{pro:interactive_multihop}, we have
\begin{equation*}
 \begin{aligned}
\prob{d(v_1,v_k) &= i} = \frac{G(k-2,k-i-1)}{\prod_{j=1}^{k-1}(2 + j(d-2))} d (d-1)^{i-1}\\
&\geq \sum_{\mathcal{I} \subset \{1, \cdots, k-2\}, |\mathcal{I}| = k-i-1}\frac{d (d-1)^{i-1}}{(k-1)d}\left(\frac{d-1}{d}\right)^{k-2}\\
&\stackrel{(a)}{=}\binom{k-2}{k-i-1}\frac{(d-1)^{i-1}}{(k-1)}\left(\frac{d-1}{d}\right)^{k-2}\\
&\geq\frac{(k-i)^{i-1}(d-1)^{i-1}}{(k-1)}\left(\frac{d-1}{d}\right)^{k-2},\\
  \end{aligned}\label{eqn:multihop}
\end{equation*}
where $(a)$ follows from the fact that the cardinality of summation is same for the number of possible ways of $k-i-1$ among $k-2$.
It is not hard to show the following inequality that
\begin{equation*}
\begin{aligned}
&\prob{v_{RC} = v_k} = I_{1/2} \left( k-1+\frac{1}{d-2}, 1+\frac{1}{d-2} \right) \\
&\quad+ (d-1) \left( I_{1/2} \left( \frac{1}{d-2}, k + \frac{1}{d-2} \right) - 1 \right)\geq \left(\frac{1}{2}\right)^{ k+\frac{1}{d-1}}.
\end{aligned}
\end{equation*}
By using these lower bound, we have
 \begin{align*}
\prob{&d(v_1,v_{RC}) = i} = \sum_{k=i+1}^\infty \text{Pr}(v_{RC} = v_k) \text{Pr}(d(v_1,v_k) = i)\\
&\geq \sum_{k=i+1}^\infty\frac{(k-i)^{i-1}(d-1)^{i-1}}{(k-1)}\left(\frac{d-1}{d}\right)^{k-2}\left(\frac{1}{2}\right)^{ k+\frac{1}{d-1}}\\
&= \alpha_d \sum_{k=i+1}^\infty\frac{(k-i)^{i-1}(d-1)^{i-1}}{4(k-1)}\left(\frac{d-1}{2d}\right)^{k-2}\\
&\geq \alpha_d \sum_{k=i+1}^\infty \frac{k^{i}}{2^k }\left(\frac{d-1}{d}\right)^i\\
&\geq  \sum_{k=i+1}^\infty\binom{k}{i}\left(\frac{1}{2}\right)^{i}\left(\frac{1}{2}\right)^{k-i}\left(\frac{d-1}{d}\right)^i\\
&\geq  \sum_{k=i+1}^\infty \frac{(k/2)^i e^{-k/2}}{i !}\left(\frac{d-1}{d}\right)^i\\
&\geq \left(\frac{d-1}{d}\right)^i\sum_{k=i+1}^\infty e^{-k/2}\geq \left(\frac{d-1}{d}\right)^{i} e^{-(i+1)},
 \end{align*}
where $\alpha_d = (1/2)^{\frac{1}{d-1}+2}$. This completes the proof of Lemma~\ref{lem:distance1}.
\end{proof}

Next, we construct the following Markov chain.
Let $\hat{p}:=\prob{W = r}$ for the identity questions \ie, there is no ``no'' answers for the
identity questions so that the algorithm should chooses one of neighbor nodes uniformly at random
and let $\hat{q}:=\prob{Z_1 (v) > Z_j
(v),~ \forall j}$ for the direction question, respectively.
Different to the case for $p=1$ which the node reveals itself as the rumor source or not
with probability one so that the Markov chain has the absorbing state, in this case, there is no such a state.
To handle this issue, we use
the information that how many times the neighbors indicate a node as its parent and how many times a node reveals itself as the rumor source.
To do that, we consider the case that there is a \emph{token}\footnote{The token keeper is regarded as the current respondent in this model.} from the initial state and
it move to the next state after additional querying follows the answer. Then this probability is the same that after $K/r$-step of Markov chain, and we expect that the rumor source $v_1$ will have the largest chance to keeping this token due to the assumption of biased answer. Let $X_n$ be the state (node) which keep this token at time $n$ where
the state is consist of all node in $V_N$. The initial state is the rumor center such that $X_0 =0$ where $0$ indicates the rumor center. Then there are $(d(d-1)^{K/r}-2)/(d-2)$ states and we can index all the state properly. Let $p^{n}_{k,j}$ be the $n$ step transition probability from the state $k$ to the state $j$.
To obtain this probabilities, we first label an index ordering by counter-clockwise from the rumor center $X_0=0$. Then, we have $P(X_{n+1} =k|X_n =k)=0$ for all $k$ and $n$, respectively. Furthermore, $P(X_{n+1} =j|X_n =k)=0$ for all $d(k,j)>1$ since the token is moved one-hop at one-step ($r$ querying). Then, the transition probability for the node $k$ which is not a leaf node in $V_L$ is as follows.
\begin{align*}
p_{k,j}=\begin{cases}
\frac{\hat{p}}{d}+(1-\hat{p})\frac{1-\hat{q}}{d-1}&\mbox{if}~j\notin nb(k,v_1)\\
\frac{\hat{p}}{d}+(1-\hat{p})\hat{q}&\mbox{if}~j \in nb(k,v_1),
\end{cases}
\end{align*}
where $nb(k,v_1)$ is the set of neighbors of the node $k$ on the path between the node $k$ and $v_1$.
%Next, let the indicator variable for a node $v \in V_l$ as $I_n (v)=1$ if $X_n =v$ and $I_n (v)=0$ if $X_n \neq v$
%which indicates that the node $v$ keeps the token at time $n$. Then, by the Markov property, we have
%\begin{equation}\label{eqn:expectation1}
%    \begin{aligned}
%     \mathbb{E}\left[\sum_{n=0}^{K/r}I_n (v)|X_0=0\right]&=\sum_{n=0}^{K/r}\mathbb{E}[I_n |X_0 =0]\\
%     &=\sum_{n=0}^{K/r}\prob{X_n= v |X_0 =0}=\sum_{n=0}^{K/r}p^{n}_{0,v}.
%    \end{aligned}
%  \end{equation}
%
%Note that the transition probability for the leaf node is slightly different from this since there is no possibility to move out of $V_l$. This implies that the transition probability becomes
%$P(X_{n+1} =j|X_n =k)=1$ for the leaf node $k$ and its parent node $j$.
%To obtain the probability in \eqref{eqn:transition}, consider that for a given $K$, this probability has non-zero only when $d(v_1, v_{RC})\leq K/r$, in other word, the transition probability $p^{n}_{0,v}$ is zero for $n< i$. Furthermore, when the distance is $i$ then there is non-zero probability for hitting this state if $n=i+2m\leq K$ where $m=0,1,2,..,M$ is an integer. Hence,
%\begin{equation}\label{eqn:t}
%    \begin{aligned}
%     \mathbb{E}\left[\sum_{n=0}^{K/r}I_n (v_1)|X_0=0\right]=\sum_{n=0}^{K}p^{n}_{0,v_1}=\sum_{n=i}^{K/r}p^{n}_{0,v_1}=\sum_{m=0}^{M}p^{i+2m}_{0,v_1},\\
%    \end{aligned}
%  \end{equation}
%where $M=\lfloor (K/r-i)/2\rfloor$.
From the simple Markov property of querying scheme, if we assume that the source node is an absorbing state then
we obtain for a given budget $K/r\geq l$,
    \begin{align}\label{eqn:transition}
     \prob{&Q(v_1)\geq1|d(v_1, v_{RC})=i}\cr
     &=1-\prob{Q(v_1)=0|d(v_1, v_{RC})=i}\cr
     &=1-\prob{\sum_{n=0}^{K}I_n (v_1)= 0|d(v_1, v_{RC})=i}\cr
     &=1-\prob{I_n (v_1)= 0,~\text{$\forall i\leq n \leq K/r$}|d(v_1, v_{RC})=i}\cr
     &=1-\prod_{n=i}^{K/r}(1-p^{n}_{0,v})\cr
     &\stackrel{(a)}{\geq}1-\prod_{n=i}^{K/r}(1-p^{K/r}_{0,v})=1-(1-p^{K/r}_{0,v})^{K/r-i}\cr
     &\stackrel{(b)}{\geq}1-e^{-(K/r -i)p^{K/r}_{0,v}},
    \end{align}
where $(a)$ follows from the fact that $p^{n}_{0,v}\geq p^{K/r}_{0,v}$ for all $i\leq n \leq K/r$ and $(b)$ is from the relation of $(1-p)^{K/r} =e^{K/r \log (1-p)}\leq e^{-p(K/r)}$ where we use the inequality $\log (1-x) \leq -x$ for $0\leq x \leq 1$. Note that the transition probability is the case of $d(v_1, v_{RC})=i$. From Lemma, we have
\begin{equation*}
    \begin{aligned}
     \prob{Q(v_1)\geq1}&\geq\sum_{i=1}^{\infty}(1-e^{-(K/r -i)p^{K/r}_{0,v}})P(d(v_1, v_{RC})=i)\\
     &\geq\sum_{i=1}^{\infty}(1-e^{-(K/r -i)p^{K/r}_{0,v}})\left(\frac{d-1}{d}\right)^{i} e^{-(i+1)}\\
    &\geq 1-ce^{-K/r p^{K/r}_{0,v}}\geq 1-ce^{-\frac{Kp}{r}  (q-1/d)^3},\\
    \end{aligned}
  \end{equation*}
where the last inequality is follows from the fact that
\end{proof}

Next, we have the following result.

\smallskip
\begin{lemma}
When $p>1/2$ and $q>1/d,$
\begin{equation*}
 \begin{aligned}
\prob{v_1 \in S_D |v_1 \in V_s} \geq 1- e^{-\frac{Kp (d-1)(q-1/d)^2}{3rd}}
   \end{aligned}
   \end{equation*}
\label{lem:directionInter}
\end{lemma}
\smallskip

\begin{proof}
\smallskip
Due to the Markov property of counting the designations from neighbors, we use following known result \cite{Markov} as
a lemma.

\smallskip
\begin{lemma}(\cite{Markov})
Let $\mathcal{X}$ denote a Markov chain with state space $E$. Then, the total number $N_j$ of visits to a state $j \in E$ from starting state $i$ under $K$ step is given by
\begin{equation}\label{eqn:hitting}
    \begin{aligned}
      \prob{N_j = m |X_0 =j}=f^{m-1}_{jj} (1-f_{jj}),
    \end{aligned}
  \end{equation}
for $i=j$ and $0 \leq m \leq K/2$. For $i\neq j$
\begin{align*}
\prob{N_{j} = m |X_{0} =i}=\begin{cases}
\qquad 1-f_{ij}&\mbox{if}~~m=0\\
f_{ij} f_{jj}^{m-1} (1-f_{jj})
&\mbox{if}~~1\leq m \leq K/2,
\end{cases}
\end{align*}
where $f_{ij}:=\prob{\tau_{j} \leq K |X_{0} = i}$. Here, $\tau_j$ is the first hitting time from starting state $i$.
\end{lemma}\label{lem:inter}
\smallskip

Hence, we see that the term $f_{ij}$ is same for the probability $\prob{Q(v_j )\geq 1 | d(v_1 , v_{RC} )=i}$ for given
budget $K$.
In our case, the initial state is $X_0 =0$ which is the rumor center then from similar steps in \eqref{eqn:transition}, we have $f_{0,v}\geq 1-e^{-(K-j)p^{K}_{0,v}}$ for node $v$ with $d(v,v_{RC})=j$. Let $N(v):=\sum_{n=0}^{K}I_n (v)$ then for all node $v \in V_l$,
\begin{equation}\label{eqn:designation}
    \begin{aligned}
     &\prob{v_1 \in S_D |d(v_1, v_{RC})=i}\\
     &=\prob{N(v_1)> N(v), \forall v \in V_l |d(v_1, v_{RC})=i}\\
     &\stackrel{(a)}{\geq}1-\sum _{v \in V_l}\left[\sum _{m=1}^{K/r}\prob{N(v)\geq  m |N(v_1)=m}\prob{N(v_1)=m}\right]\\
     &=1- n_1\sum _{m=1}^{K/r}\prob{N(v)\geq m |N(v_1)=m}\prob{N(v_1)=m}\\
     &=1- n_1\sum _{m=1}^{K/r}\left(\sum _{j=m}^{K/r}\prob{N(v)=j}\right)\prob{N(v_1)=m}\\
     &\stackrel{(b)}{\geq}1- n_1\sum _{m=1}^{K/r}e^{-mK}\prob{N(v_1)=m}\stackrel{(c)}{\geq} 1-ie^{-\frac{Kp (d-1)(q-1/d)^3}{rd} },
    \end{aligned}
  \end{equation}
where $(a)$ is from the union bound of the joint probability and the inequality $(b)$ is from the fact that $\sum _{j=m}^{K/r}\prob{N(v)=j} \leq e^{-mK}$ where $n_1$ is the number of queried nodes in $V_s$.\footnote{The number of visiting for any state can not beyond $K/r$ in the policy.}
The last inequality $(c)$ is from the geometric sum of $e^{-mK}$ with mean of binomial distribution $Kp$.
The probability $f_{ij}$ for a node $v$ can be obtain by considering (1) distance from $v_{RC}$ ($d(v,v_{RC})=i$) and (2) indication whether it is on the path between rumor center and source because the transition probability will be different.
Then, using this result, we have
    \begin{align*}
  \prob{v_1 &\in S_D |v_1 \in V_s}\\
  &=\sum_{i=0}^{l}\prob{v_1\in S_I |d(v_1, v_{RC})=i}\prob{d(v_1, v_{RC})=i}\\
  &\geq \sum_{i=0}^{l} \left(1-ie^{-\frac{Kp (d-1)(q-1/d)^3}{rd} }\right) \left(\frac{d-1}{d}\right)^{i} e^{-(i+1)}\\
  &= \sum_{i=0}^{l} \left(1-ie^{-\frac{Kp (d-1)(q-1/d)^3}{rd} }\right) \left(\frac{d-1}{ed}\right)^{i} \frac{1}{e}\\
    &\stackrel{(a)}{\geq} \sum_{i=0}^{l} \left(1-ie^{-\frac{Kp (d-1)(q-1/d)^3}{rd} }\right) \left(\frac{1}{3}\right)^{i+1}\\
    &\stackrel{(b)}{\geq} 1- e^{-\frac{Kp(d-1)(q-1/d)^2}{3rd}},
    \end{align*}
where $(a)$ is from the fact that $\left(\frac{3(d-1)}{ed}\right)^i >\frac{e}{3}$ for all $0 \leq i \leq l$
and $(b)$ comes from some algebra using the geometric sum for the $i.$
Hence, this completes the proof of Lemma \ref{lem:directionInter}.
\end{proof}

Similar to the previous one, to obtain the detection probability, we need to find the probability $P(v_1 \in S_N \cap S_I|v_1 \in V_s)$.
From this, we consider $r$ repetition count for identity question and $r-X_{r}(v)$ for direction question where $(X_{r}(v)$
be the number of yes answers of the queried node $v$ with probability $p_v$. Hence, we see that the number of repetition count
for the direction questions is also a random variable which follows a binomial distribution with parameter $p_v$.
By considering this, We have the following lemma.

\smallskip
\begin{lemma}
Suppose $v_1 \in V_l$ then we have
\begin{equation}\label{eqn:candidate}
    \begin{aligned}
      P(v_1 \in S_I \cap S_D |v_1 \in V_s)\geq 1-e^{-3g(p,q)^2 (K/r)\log r},
    \end{aligned}
  \end{equation}
where $g (p,q)=\frac{2d}{d-1} (p-1/2)^2 + \frac{d-1}{d-2} (q-1/d)^3$.
\label{lem:filter_Inter}
\end{lemma}
\smallskip

\begin{proof}
Since the events $v_1 \in S_I$ and $v_1 \in S_D$ are independent for a given $v_1 \in V_s$,
by using lemma \ref{lem:directionInter} and \ref{lem:directionInter} and some algebra, we have
\begin{equation*}
    \begin{aligned}
      &\prob{v_1 \in S_I \cap S_D |v_1 \in V_s}\\
      &\geq \left(p+(1-p)(1-e^{-p^{2}\log r})\right) \left(1-ce^{-\frac{Kp}{r}  (q-1/d)^3}\right)\\
      &\qquad \cdot \left(1- e^{-\frac{K (d-1)(q-1/d)^2}{3rd}}\right)\\
      &\geq  1-e^{-3g(p,q)^2 (K/r)\log r},
    \end{aligned}
  \end{equation*}
where $g (p,q)=c_1 (p-1/2)^2 + c_2 (q-1/d)^3$ for some constants $c_1$ and $c_2$ which are only depends on the degree $d$. This completes the proof of Lemma~\ref{lem:filter_Inter}.
\end{proof}

Next, we consider the following lemma which indicates the lower bound of detection probability
among the final candidate set.

\smallskip
\begin{lemma} \label{lem:filtration1}
  When $d\geq3$, $p>1/2$ and $q>1/d$,
  \begin{eqnarray*}
    \prob{v_1 =v_{LRC}|v_1 \in S_I \cap S_D}  & \geq & 1-e^{-g(p,q) r\log r}.
  \end{eqnarray*}
\end{lemma}
\smallskip

The proof technique is similar to the Lemma \ref{lem:filtration} so we omit it.
Using the obtained lemmas 5-8, we finally get the lower bound of detection probability
 of {\bf MVAD}$(r)$ for a given repetition count $r$ and this completes the proof of
 Lemma~\ref{lem:inter_prob}.
\end{proof}

The term $g_d (r,q)$ in
\eqref{eqn:detect2} is the probability that the
respondent reveals the true parent for given $r$ and $q$.
 Hence, one can see
 that for a fixed $K$, large $r$ leads to the increasing this
 probability due to the improvement for the quality of the direction answer.
 However, increasing $r$
 negatively affects the term $K/(r+1)$ in \eqref{eqn:detect2}, so that
 there is a trade off in selecting a proper $r$. The detailed proof will be
provided in our technical paper\cite{Jae16}.
By considering the error probabilities, we obtain
\begin{equation}\label{eqn:error}
\begin{aligned}
\prob{\hat{v}\neq v_{1}}&\leq
c \cdot e^{- (K/r)\log (K/r)}+e^{-3g(p,q)^2 (K/r)\log r}\\
&+e^{-g(p,q) r\log r}\\
&\stackrel{(a)}{\leq}( c
+1)e^{-2g(p,q)^2 (K/r)(\log K/r)},
\end{aligned}
\end{equation}
where $c_1=c+1$ and the inequality $(a)$ is from the fact that
$g(p,q) <1$.
By derivation of the result with respect to $r$, we first obtain $r^*$ which maximizes the detection
probability by $r^*= \left\lfloor1+\frac{7d^2 \{2(1-p)^3 + (1-q)^2\} \log\log
  K}{3(d-1)}\right\rfloor$ in {\bf MVAD}$(r^*)$
and put this into the error probability $\prob{\hat{v}\neq v_{1}}$, we have
\begin{align}\label{eqn:choi}
\prob{\hat{v}\neq v_{1}}&\leq
( c
+1)e^{-2g(p,q)^2
  (K/(r^*))\log(K/(r^* ))}\cr
   &\stackrel{(a)}{\leq} ( c
+1)e^{-g (p,q) K^2
  \log(K/(r^*))}\cr
 &\stackrel{(b)}{\leq} ( c
+1) e^{-g (p,q)K\log (\log K)},
\end{align}
where the inequality $(a)$ is from the fact that $K\log (K/(r^*))>\log K$ and $(b)$
comes from the obtained result of $r^*$. Let
$\delta \geq ( c
+1) e^{-f_2 (p,q)K\log (\log K)},$ then, we obtain the value of $K$ which
 produces the error probability $\delta$ in later and we obtain the
desired lower-bound of $K$ as in the theorem statement. This completes
the proof.

\begin{figure*}
\subfigure[Characterization of $\prob{d(v_1,v_k)=1}$.
]{\includegraphics[width=0.35\textwidth]{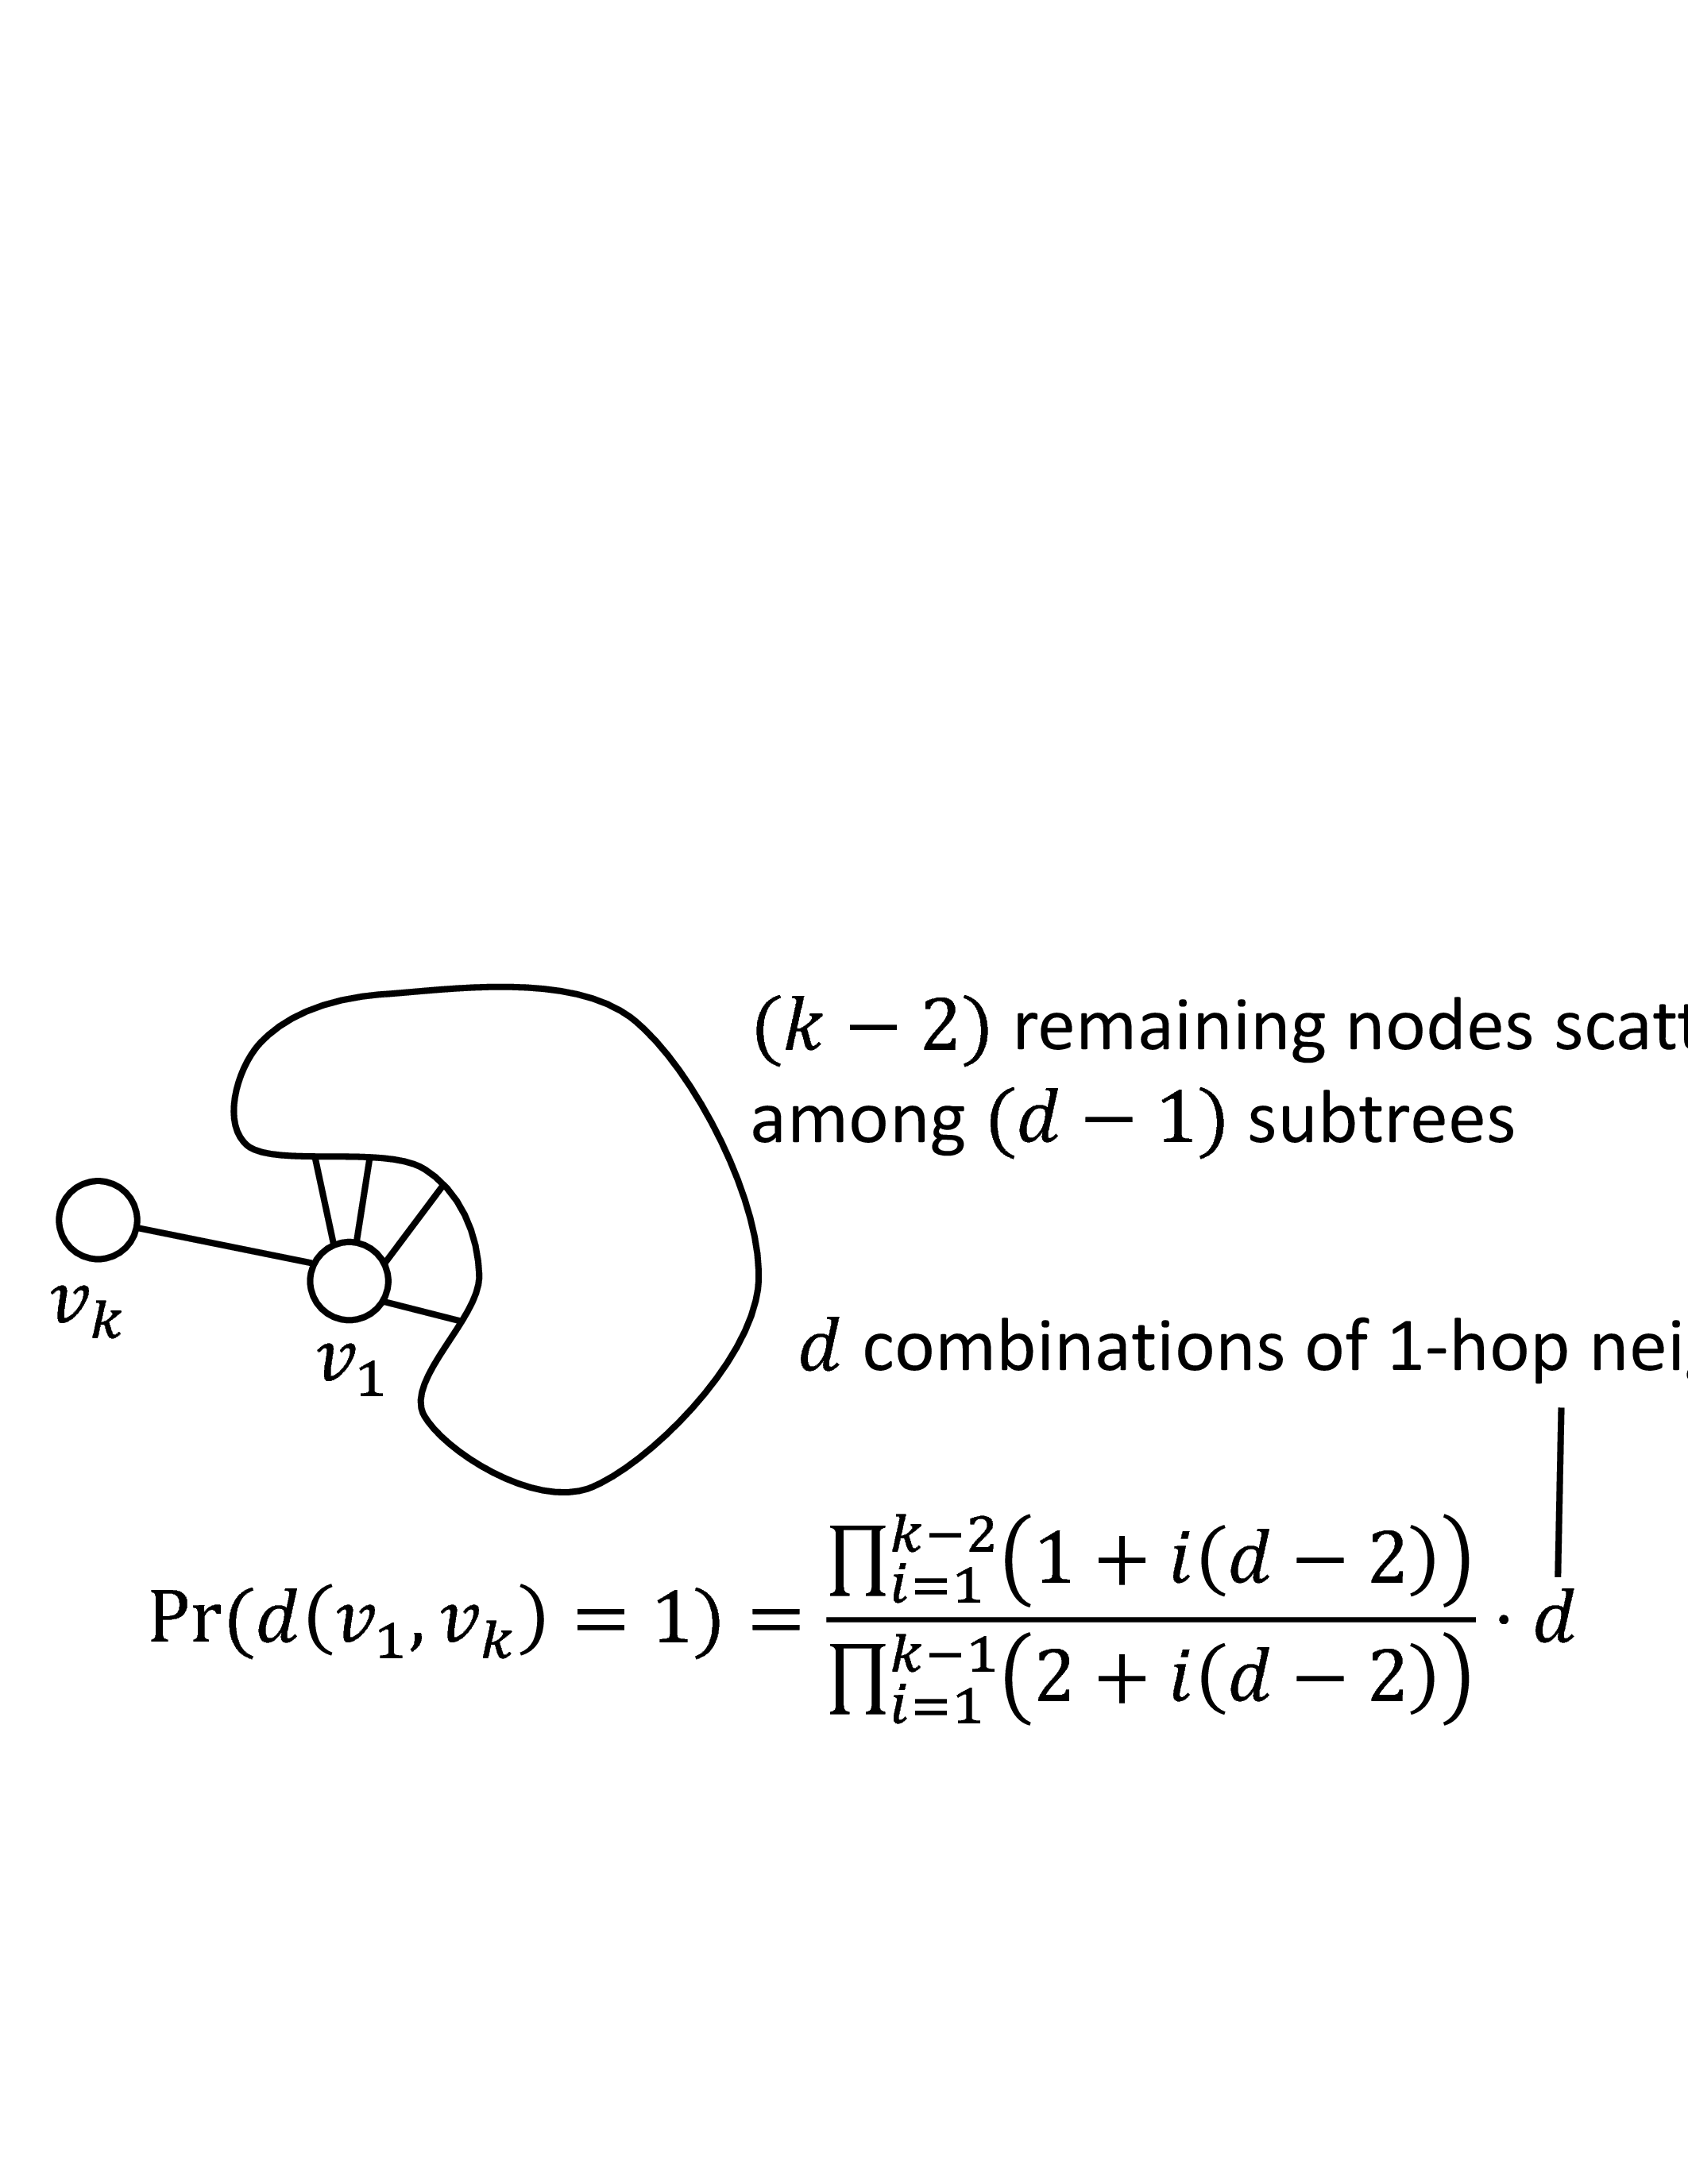}\label{fig:interactive_1hop}}
\subfigure[Example for $d(v_1,v_6)=3$.
]{\includegraphics[width=0.21\textwidth]{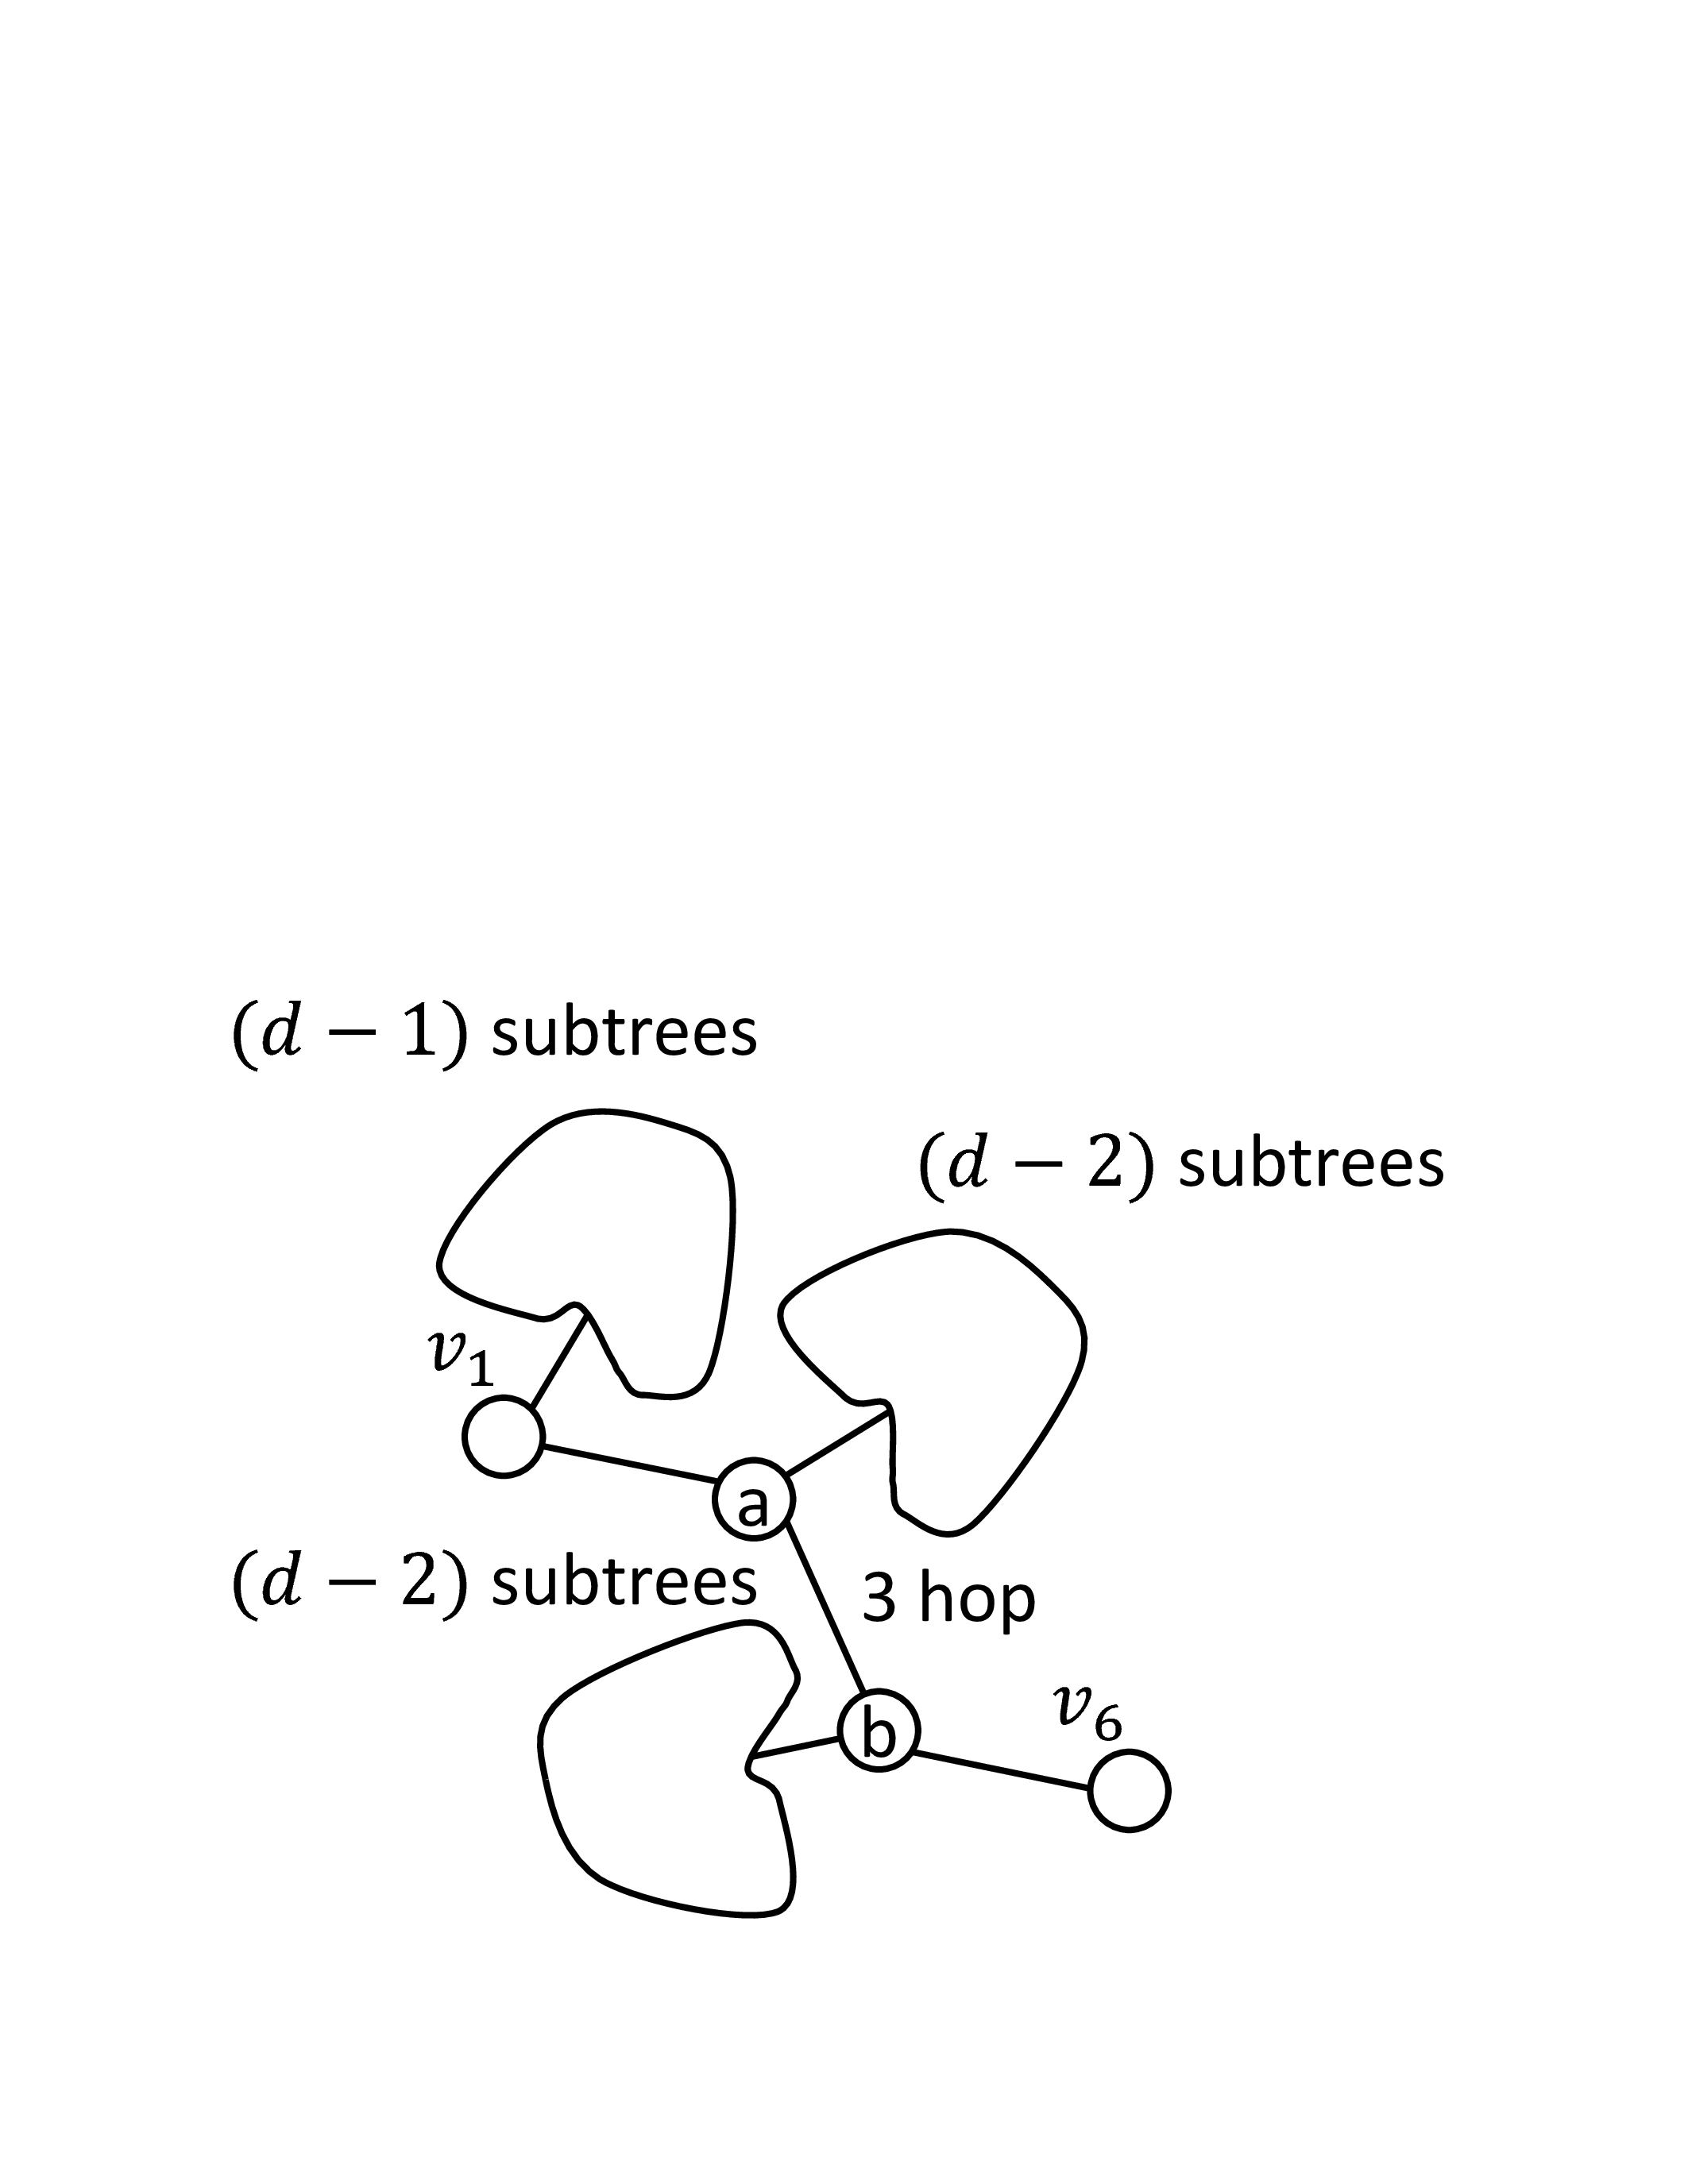}\label{fig:interactive_multihop_a}}
\subfigure[Case I.
]{\includegraphics[width=0.21\textwidth]{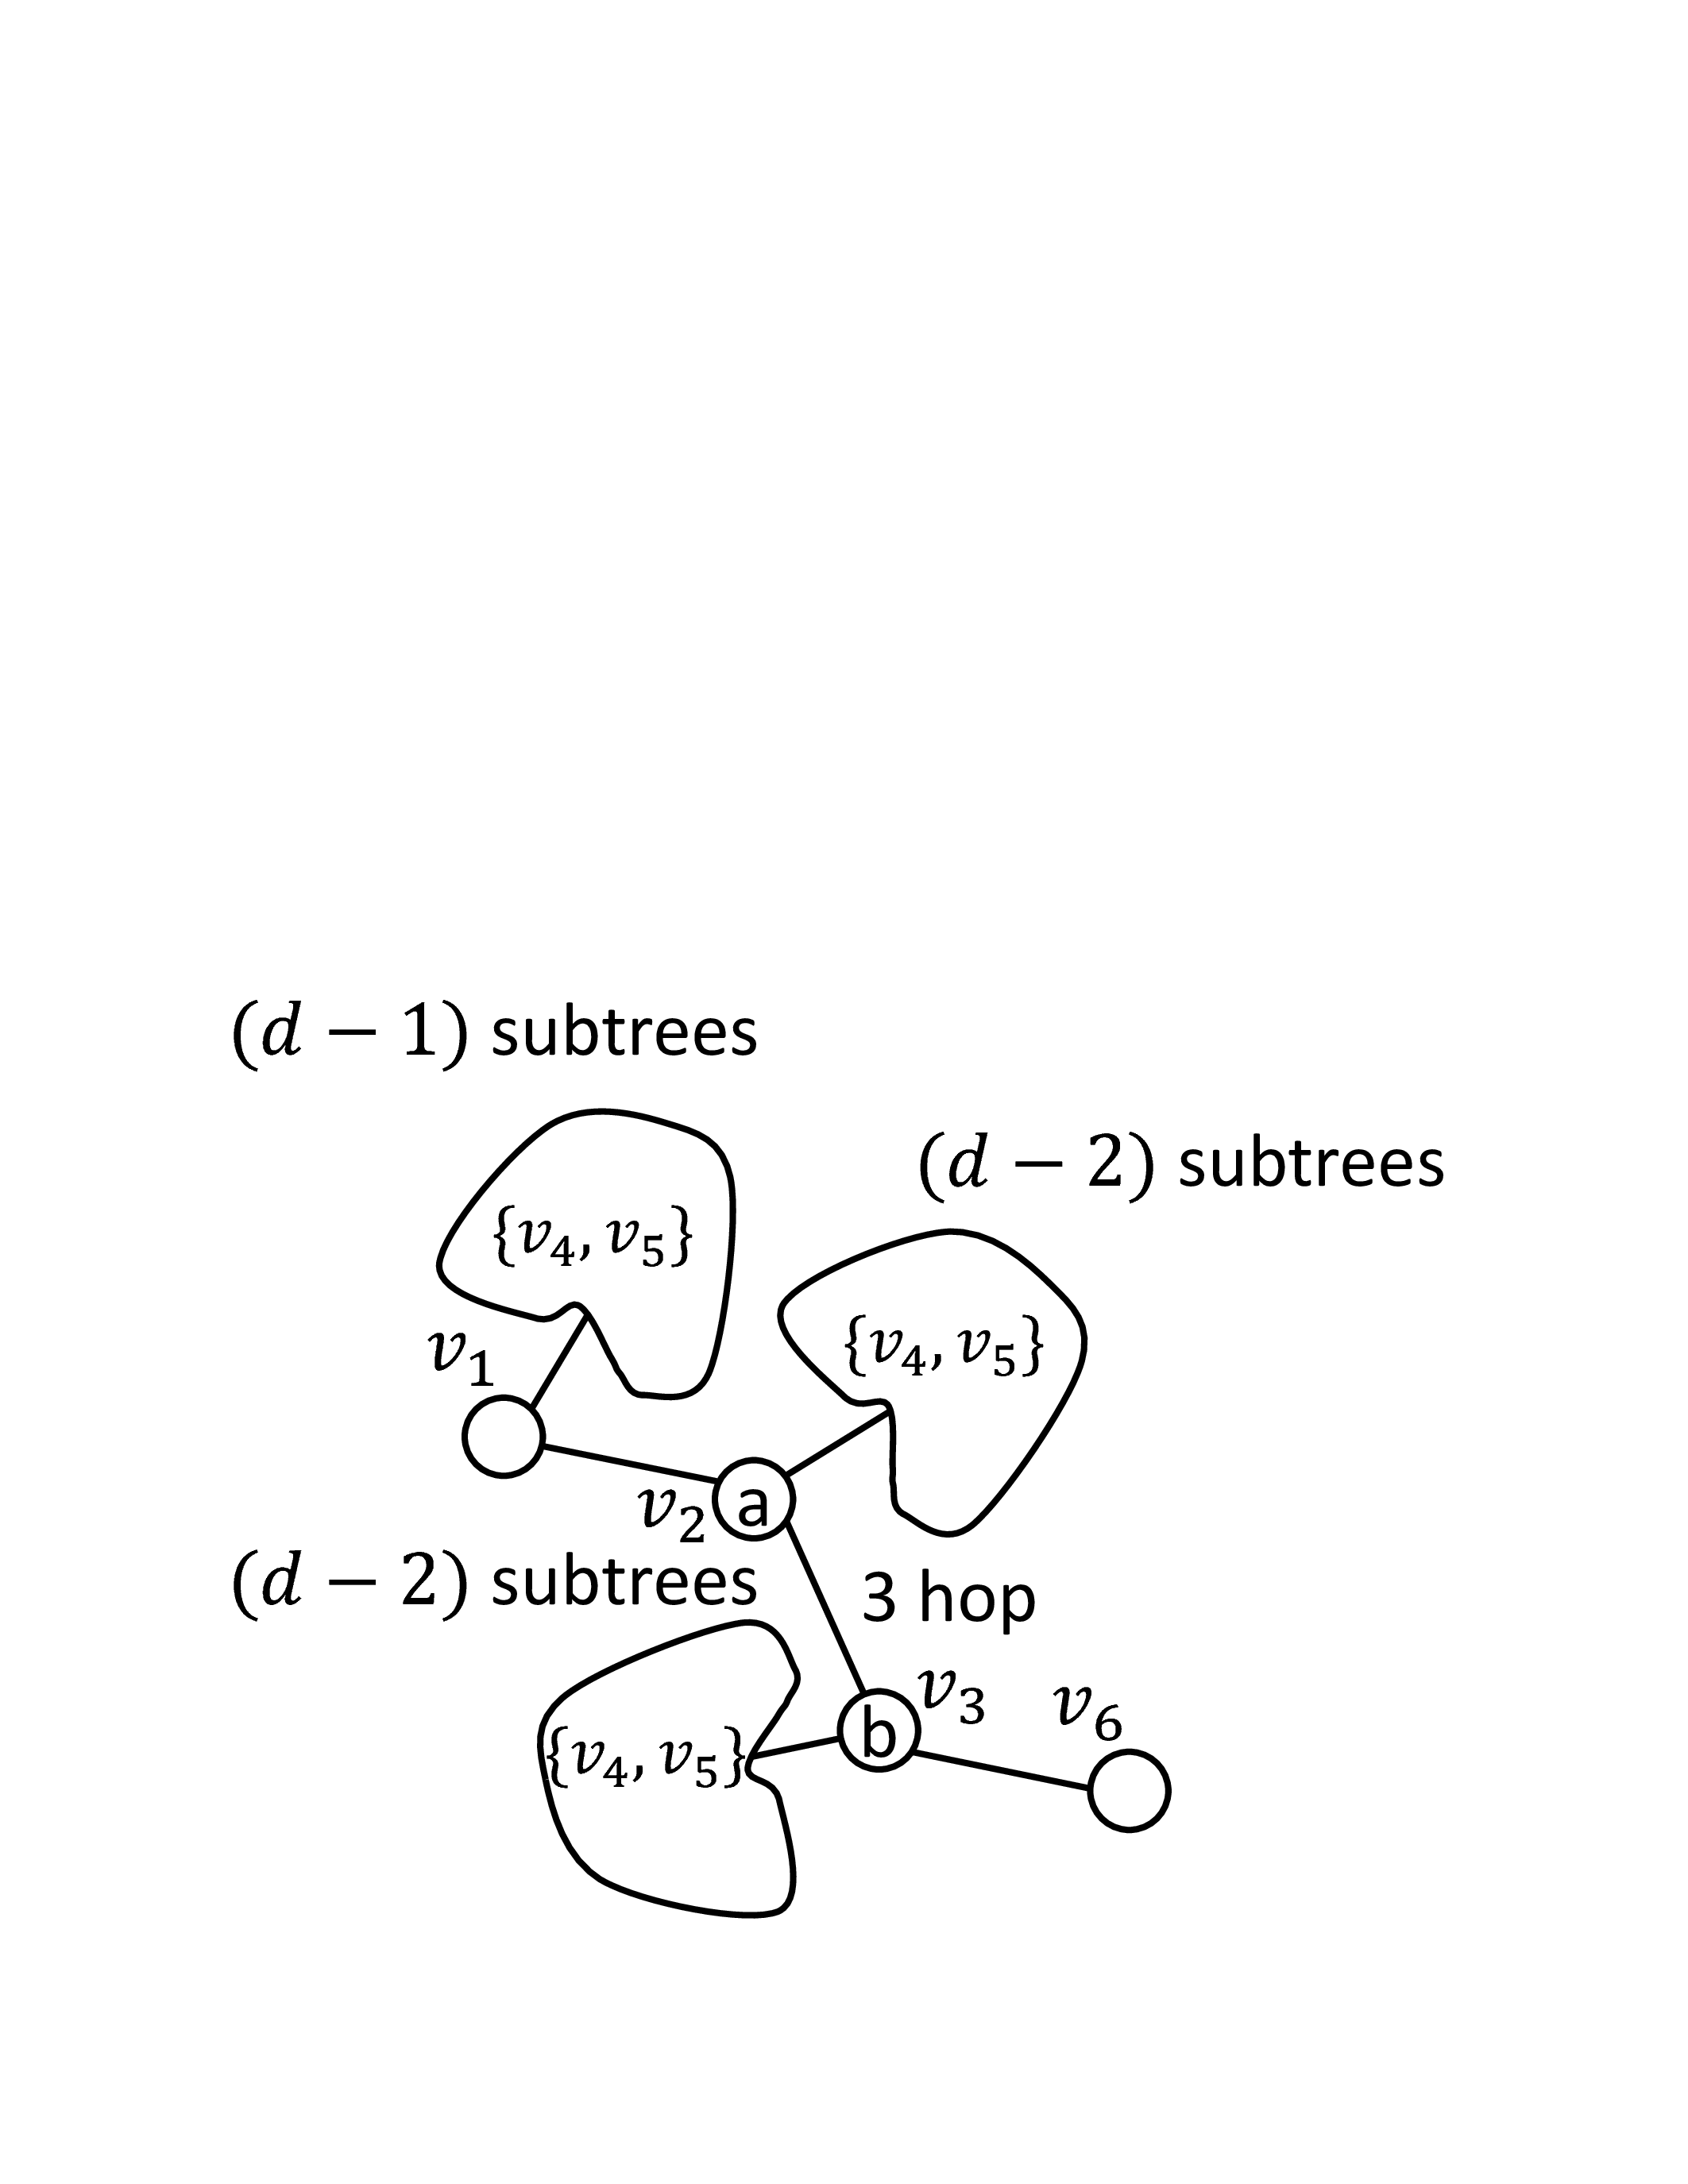}\label{fig:interactive_multihop_b}}
\subfigure[Case II.
]{\includegraphics[width=0.21\textwidth]{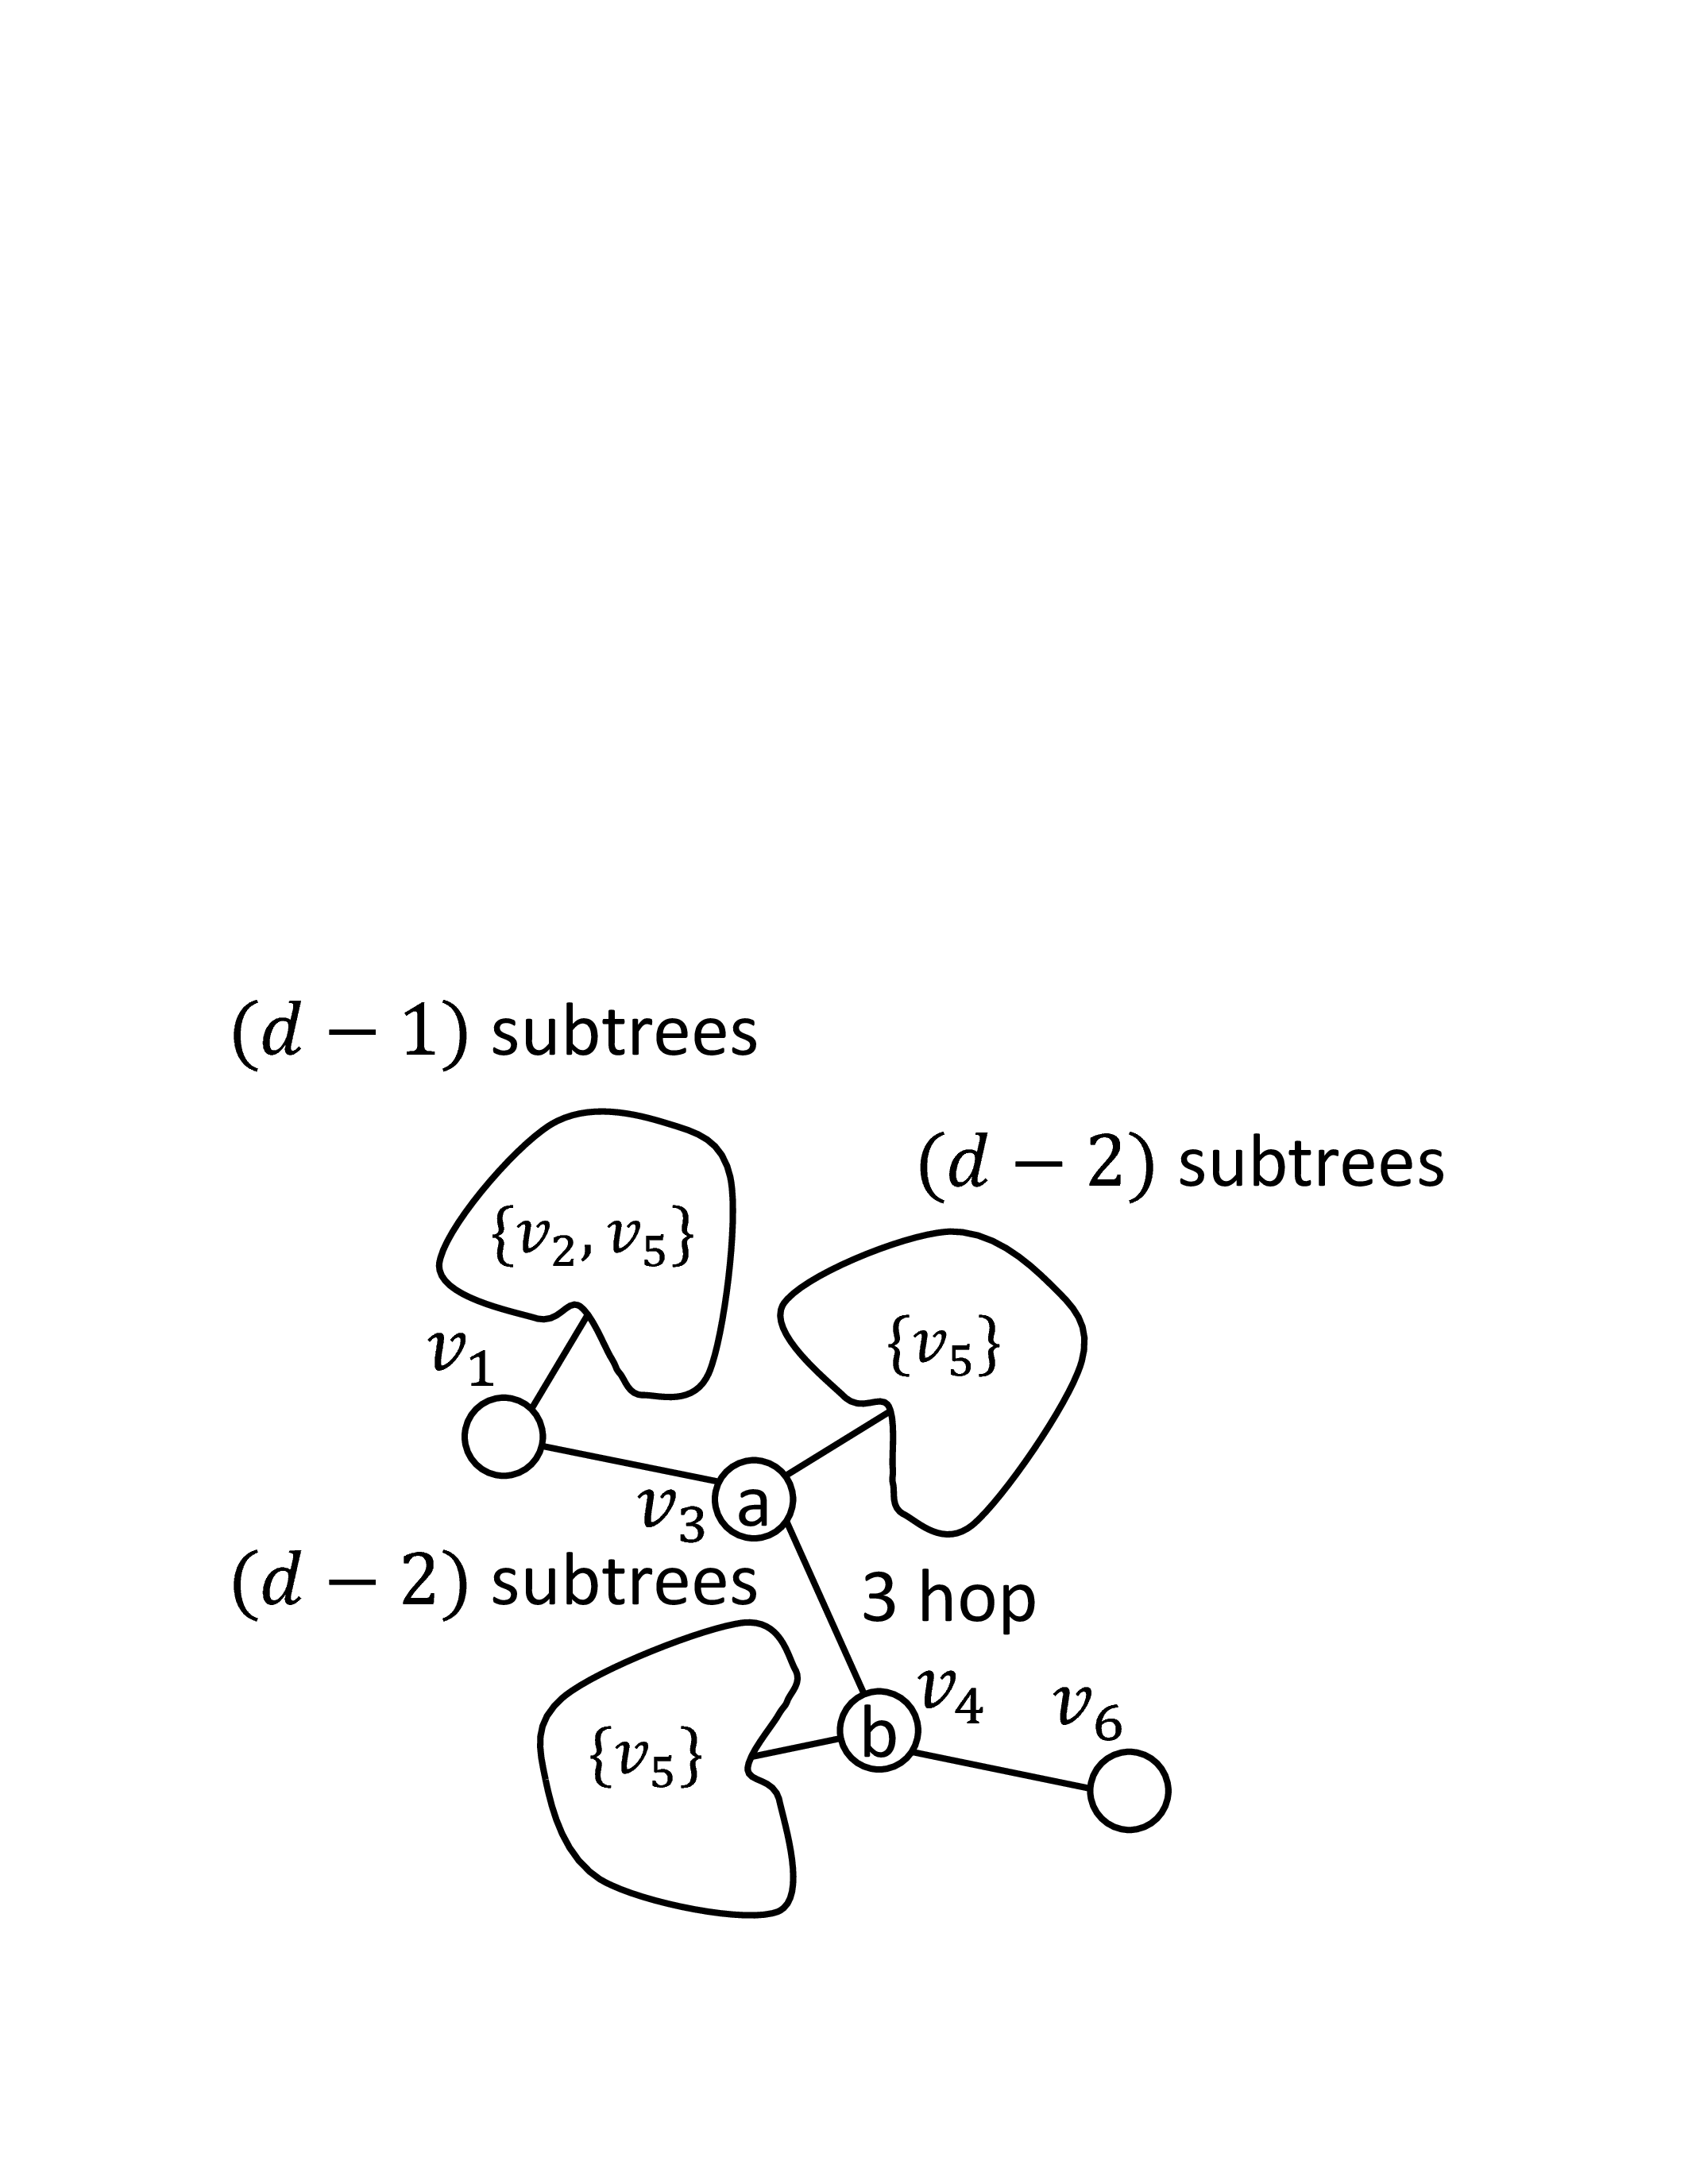}\label{fig:interactive_multihop_c}}
\caption{Illustrative example of deriving (a) $\prob{d(v_1,v_k)=1}$ and (b)(c)(d) $\prob{d(v_1,v_k)=i}$ when $k=6$ and $i=3$.}
%\label{fig:interactive_multihop}
\end{figure*}

\subsection{Proof of Proposition \ref{pro:interactive_multihop}}
For simple understanding, we first see the case for single-hop distant which
is more simple than that of general case. Consider $d(v_1,v_{RC}) \leq 1$, that the rumor source is within the one-hop
distant from the rumor center and for this case, the required number of budget is $K=1$ \footnote{First, the algorithm chooses
the rumor center as an MLE and perform the query if she is not the source for the direction question.}
. To obtain the detection probability, we consider the following lemma.
\begin{proposition}
The detection probability when $K=1$ is given by
\begin{equation*}
\begin{aligned}
\prob{\hat{v}=v_{1}}=\prob{v_1 = v_{RC}} +
q\cdot\prob{d(v_1,v_{RC}) = 1},\\
\end{aligned}
\end{equation*}
where
\begin{equation*}
\prob{d(v_1,v_{RC})=1} = \sum_{k=2}^{\infty} \prob{ d(v_1,v_k)=1 } \prob{ v_k = v_{RC} },
\end{equation*}
and
\begin{equation*}
\prob{d(v_1,v_k)=1} = \frac{\prod_{i=1}^{k-2}(1+i(d-2))}{\prod_{i=1}^{k-1}(2+i(d-2))} \cdot d.
\end{equation*}

\label{pro:interactive_singlehop}
\end{proposition}

Next, from the single-hop distant case, we extend the result to multi-hop extant case as follows.
From \cite{shah2012}, the first term $\prob{v_1=v_{RC}}$ can be directly obtained so it remains
to find the second term $\prob{d(v_1,v_{RC})=1}$.  To obtain this, we will
decompose the event $\{d(v_1,v_{RC})=1\}$ by
disjoint events, considering subcases where $v_{RC} = v_k$ for
different $k$. Because the rumor center becomes a single node in
case of $N \rightarrow \infty$, the event $\{v_{RC} = v_k\}$ can be decomposed
into disjoint sub-events.  First, let's consider the case when
$v_{RC}=v_2$. Then, it is clear that $d(v_1,v_2)=1$ because $v_1$ and
$v_2$ are always adjacent. In case of $v_{RC} = v_k$ for $k\geq 3$, $v_k$
is not always adjacent to $v_1$, and therefore we express
$\prob{d(v_1,v_{RC})=1}$ as
  \begin{equation*}
    \begin{aligned}
      \prob{d(v_1,v_{RC})=1} &= \sum_{k=2}^{\infty} \prob{ v_{RC}=v_k, d(v_1,v_k)=1 } \\
      &\stackrel{(a)}{=}\sum_{k=2}^{\infty} \prob{ v_{RC}=v_k } \prob{ d(v_1,v_k)=1 },
    \end{aligned}
  \end{equation*}
where the equality $(a)$ holds because for all $k\geq 2$, the events
  $\{v_{RC}=v_k\}$ and $\{d(v_1,v_k)=1\}$ are independent. This can be
  explained from the fact that $\{d(v_1,v_k)=1\}$ is caused from the
  first $k$ infections, and $\{v_{RC}=v_k\}$ is occurred from
  \emph{beyond} $k$th infection, which makes there are no causal
  relationships between two events.  \footnote{More formally, we can
    make the condition $\{d(v_1,v_k)=1\}$ and derive
    $\prob{v_k = v_{RC} | d(v_1,v_k)=1}$.  The topology of first
    $k$ infected nodes has no role to determine the entire ratio of
    subtree sizes since all of first $k$ infected nodes reside on a
    same subtree.  This makes
    $\prob{v_{RC}=v_k | d(v_1,v_k)=1} = \prob{v_k=v_{RC}}$.}
  From
  \cite{shah2012}, the probability $\text{Pr}(v_{RC}=v_k)$ is given by
  \begin{equation*}
\begin{aligned}
\prob{v_{RC} = v_k} &= I_{1/2} \left( k-1+\frac{1}{d-2}, 1+\frac{1}{d-2} \right) \\
&+ (d-1) \left( I_{1/2} \left( \frac{1}{d-2}, k + \frac{1}{d-2} \right) - 1 \right).
\end{aligned}
\end{equation*}
Therefore, we only need to characterize
  $\prob{d(v_1,v_k)=1}$.
To obtain this, we need to count two kinds of permutations,
(i) the total number of possible topological realizations of
$\{v_1,\cdots,v_k\}$, (ii) the number of realizations of
$\{v_1,\cdots,v_k\}$ satisfying $d(v_1,v_k)=1$.
Fig.~\ref{fig:interactive_1hop} describes the evaluation of
the probability.
\begin{enumerate}[(i)]
\item The total number of possible realizations is given by
$d (d + (d-2)) (d + 2(d-2)) \cdots (d + (k-2)(d-2))
= \prod_{i=1}^{k-1}(2 + i(d-2))$, since there are
$d$ possible subtrees around $v_1$ to locate remaining nodes.
\item The total number of realizations where $d(v_1,v_k)=1$
can be counted as follows. First we fix $v_1$ and $v_k$ as
one-hop neighbor, then we place remaining nodes $\{v_2,\cdots,v_{k-1}\}$
around $(d-1)$ subtrees around $v_1$. This makes
$(d-1)((d-1)+(d-2))((d-1)+2(d-2))\cdots((d-1)+(k-3)(d-2))
= \prod_{i=1}^{k-2}(1+i(d-2))$.
Then we multiply this number by $d$ since there are $d$ possible ways
to place $v_1$ and $v_k$ adjacently.
\end{enumerate}
Since all permutation have the equal probability due to the exponential distribution under regular tree,
we obtain the probability Pr($d(v_1,v_k)=1$) as
\begin{equation*}
\prob{d(v_1,v_k)=1} = \frac{\prod_{i=1}^{k-2}(1+i(d-2))}{\prod_{i=1}^{k-1}(2 + i(d-2))}
\cdot d.
\end{equation*}
This completes the proof of Proposition~\ref{pro:interactive_singlehop}.

In this subsection, we will provide the derivation of \eqref{eqn:interactive_multihop}.
Different to the case $i=1$, the probability $\prob{d(v_1,v_k)=i}$ has more complex and general
form. To find this, we first define $G(a,b)$ for given $a\in Z_+$ and $b\in Z$ such that
\begin{equation*}
\begin{aligned}
G(a,b) &\triangleq& \sum_{\mathcal{I} \subset \{1, \cdots, a\}, |\mathcal{I}| = b} \left(\prod_{i \in \mathcal{I}} x_i\right),
\end{aligned}
\end{equation*}
where $\mathcal{I}$ is any subset of $\{1, \cdots, a\}$ with cardinality $|\mathcal{I}| = b$ and $x_i = 1 + i(d-2)$.
For example, $G(a,0) = 1$ and $G(3,2) = x_1 x_2 + x_2 x_3 + x_3 x_1$.
% and $G(a,b)$ has a recurrence form as
% $G(a,b) = G(a-1, b-1) x_a + G(a-1, b)$ from the combinatorial
% property.
Note that \eqref{eqn:interactive_multihop} can be described
as the case when $i=1$, since
$G(k-2,k-2) = x_1 x_2 \cdots x_{k-2} = \prod_{i=1}^{k-2}(1+i(d-2))$.
For the more precisely understanding of $G(k-2,k-i-1)$ in
\eqref{eqn:interactive_multihop}, consider the illustrative following
example when $k=6, i=3$.  Note that all we have to do is just counting the number of
possible topologies satisfying $d(v_1,v_6)=3$.
Fig.~\ref{fig:interactive_multihop_a}-
\ref{fig:interactive_multihop_c}
show the example of deriving
$\text{Pr}(d(v_1,v_6)=3)$. Fig.~\ref{fig:interactive_multihop_a} shows
one possible realization partially satisfies the conditions.  Here in
nodes $a$ and $b$, nodes among $\{v_2,v_3,v_4,v_5\}$ can be placed,
making $\binom{k-2}{k-i-1} = \binom{4}{2}$ possible node placements.
After dividing into sub-cases, we consider the number of possible
topologies one by one.

\begin{itemize}
\item {\bf Case I:} In Fig.~\ref{fig:interactive_multihop_b}, the
  remaining unplaced nodes $\{v_4,v_5\}$ can be placed in any
  subtrees, since they are all infected after both $v_2$
  and $v_3$ are infected. The node $v_4$ can be placed among $((d-1)+2(d-2))$ subtrees, and
  this placement makes $(d-2)$ additional subtrees.  So the node $v_5$ can be
  placed among $((d-1)+3(d-2))$ subtrees.  This makes the number of
  possible topologies $(1+3(d-2))(1+4(d-2)) = x_3 x_4$ in
  Fig.~\ref{fig:interactive_multihop_b}.
\item {\bf Case II:} We can apply the similar argument in the subcase
  stated in Fig.~\ref{fig:interactive_multihop_c}.  In this case,
  among remaining nodes $\{v_2,v_5\}$, the node $v_2$ can be placed in only
  first subtree since $v_3$ is ``blocking'' the infection path and
  $v_2$ cannot be located beyond $v_3$. The node $v_5$ can be placed in any
  subtrees. This makes the number of possible topologies
  $(d-1)(1+4(d-2)) = x_1 x_4$ by considering similar combinatorics
  as in Fig.~\ref{fig:interactive_multihop_b}.
\end{itemize}
From above subcases, we can infer that there are
$x_1 x_2 + x_1 x_3 + x_1 x_4 + x_2 x_3 + x_2 x_4 + x_3 x_4 = G(4,2)$
possible realizations when the location of $v_1$ and $v_6$ are
fixed. Fixing the location of $v_1$, the node $v_6$ can be placed among
$d(d-1)(d-1) = d(d-1)^2$ possible positions. This makes the overall
$G(4,2) \cdot d(d-1)^2$ possible topologies. In general, one can easily obtain
  \begin{equation*}
\begin{aligned}
\#~of~ possible~ &topologies\\
&=G(k-2, k-i-1) \cdot d(d-1)^{i-1}.
\end{aligned}
\end{equation*}
%the
%number of possible topologies are $G(k-2, k-i-1) \cdot d(d-1)^{i-1}$.
The denominator of \eqref{eqn:interactive_multihop} is same as
the that of single-hop case, which refers the number of possible
topological realizations of $k$ infections. This conclude the proof
of Proposition~\ref{pro:interactive_multihop}.

%%%% Local Variables:
%%%% mode: latex
%%%% TeX-master: "main"
%%%% End:

\subsection{Deriving $r^*$ in \eqref{eqn:lower}}

First, for given $K,r$ and $d$, we define
\begin{equation*}
\begin{aligned}
s_{d}(K,r,p,q):&=c\cdot e^{-\frac{\log\left(\frac{K}{r}\right)}{\log(d-1)}\log \frac{\log\left(\frac{K}{r}\right)}{\log(d-1)}} \cr
     & - \frac{K((1-H(p))+p (1-p)(1-H(q)))}{\frac{K}{r}(\frac{K}{r}-1)\log \frac{K}{2r}}\cr
     & : = s_{d}^{1}(K,r) - s_{d}^{2}(K,r,p,q)
\end{aligned}
\end{equation*}
where $c = 4d/(d-1)$. To obtain $\frac{\partial s_{d}(K,r,p,q)}{\partial r}=0,$ first consider that
\begin{equation*}
\begin{aligned}
\frac{\partial s_{d}^{1}(K,r)}{\partial r}= \frac{c (K/r)^{-\frac{\log \left(\frac{\log (K/r)}{\log (d-1)}\right)}{\log(d-1)}\left(\log \left(\frac{\log (K/r)}{\log (d-1)}\right)+1\right)}}{r \log (d-1)},
\end{aligned}
\end{equation*}
and we also have that
\begin{equation*}
\begin{aligned}
\frac{\partial s_{d}^{2}(K,r,p,q)}{\partial r}=\frac{h(p,q)K^2 \log(K/2r) +K -1}{(K-r)^2 \log^2 (K/2r)},
\end{aligned}
\end{equation*}
where $h(p,q)=((1-H(p))+p (1-p)(1-H(q)))$. By setting $\frac{\partial s_{d}^{1}(K,r)}{\partial r}=\frac{\partial s_{d}^{2}(K,r,p,q)}{\partial r}$ and
after some algebra, we obtain
\begin{equation*}
\begin{aligned}
\log r \simeq \log \left ( 1+\frac{4 (1-p)\{7H(p)+H(q)\}\log K}{3e\log(d-1)}\right),
\end{aligned}
\end{equation*}
which implies that $r^{*}=\Theta\left(\frac{4 (1-p)\{7H(p)+dH(q)\}\log K}{3e\log(d-1)}\right)$ and this completes the proof.
%\subsection*{A.8. Proof of Proposition \ref{pro:difference}}
%
%To prove this, let $|C^* \cap C_L |=t$ then we have $K-t$ nodes which are in only one of the set.
%Consider a node $v \in  C^* / C_L$ or $v \in  C_L / C^*$ then we have
%\begin{align*}\label{eq:2}
%|\prob{v_1 \in C^*}-\prob{v_1 \in C_L}|&=\sum_{v \in \tilde{C}}\prob{v = v_1 }\\
%& \stackrel{(a)}{\leq} \sum_{v \in \tilde{C}} e^{-\eta_1 K}\\
%& \stackrel{(b)}{\leq}  e^{-\eta K},
%\end{align*}
%where $(a)$ follows from the fact that the probability of a node which is not in $C_L$ being the source
%$\prob{v= v_1 }\leq e^{-\eta_1 K}$ and the inequality $(b)$ is from the fact that \note{Complete this proof !}

\subsection{Deriving $r^*$ in \eqref{eqn:detect}}

First, for given $K,r$ and $d$, we define
\begin{equation*}
\begin{aligned}
f_{d}(K,r,p,q):&=c\left(\frac{r+p+q}{r+2}\right)^3\cdot
  \exp\Bigg( \frac{-h_d
  (K,r)w_d (p,q)}{2}\Bigg),
\end{aligned}
\end{equation*}
where $c = 7(d+1)/d$ and $w_d (p,q)=\frac{1}{2}(4(p-1/2)^2+(d/(d-1))^3 (q-1/d)^3)$.
The term $h_d (K,r)$ is given by
$$h_d (K,r):=\frac{\log\left(\frac{K}{r}\right)}{\log(d-1)}\log\left(
\frac{\log\left(\frac{K}{r}\right)}{\log(d-1)}\right).$$
Then one can check that this is a differential unimodular function
with respect to $r$.  Hence, by taking derivative with respect to $r$
to obtain the optimal choice of $r$, we have
\begin{equation*}
\begin{aligned}
&\frac{\partial f_{d}(K,r,p,q)}{\partial r}\\
&=\frac{\partial}{\partial
  r}\left(\frac{r+p+q}{r+2}\right)^3\left(c\cdot \exp\Bigg( \frac{-h_d
  (K,r)w_d (p,q)}{2}\Bigg)\right)\\ &\quad +
\left(\frac{r+p+q}{r+2}\right)^3\frac{\partial}{\partial
  r}\left(c\cdot \exp\Bigg( \frac{-h_d
  (K,r)w_d (p,q)}{2}\Bigg)\right).
\end{aligned}
\end{equation*}
To finish this, we first consider that
$\frac{\partial}{\partial
  r}\left(\frac{r+p+q}{r+2}\right)^3=-\frac{3(p+q-2)(p+q+r)^2}{(r+1)^4},$
and
\begin{equation*}
\begin{aligned}
&\frac{\partial (c\cdot exp\left(-h_d (K,r)w_d (p,q)/2\right))}{\partial
  r}\\
&=\frac{c(K/r)^{\frac{-\log(Q_d (K,r) w_d (p,q))}{\log(d-1)}}(\log Q_d
  (K,r) w_d (p,q)+1)}{2r\log(d-1)},
\end{aligned}
\end{equation*}
where $Q_d (K,r)=\log (K/r)/\log(d-1).$ From the relation $h_d
(K,r)=Q_d (K,r)\log(Q_d (K,r))$ and $\frac{\partial
  f_{d}(K,r,p,q)}{\partial r}=0$, we have
\begin{equation*}
\begin{aligned}
&\frac{3(p+q-2)(p+q+r)^2}{(r+1)^4}\\
&\qquad=\frac{c(K/r)^{\frac{-\log(Q_d
      (K,r)w_d (p,q))}{\log(d-1)}}(\log Q_d (K,r)w_d (p,q)+1)}{2r\log(d-1)\left(1-1/Q_d
  (K,r)^{Q_d (K,r)})\right)}\\
&\qquad \simeq \frac{c(K/r)^{\frac{-\log(Q_d
      (K,r))}{\log(d-1)}}\log Q_d (K,r)w_d (p,q)}{2r\log(d-1)}.\\
\end{aligned}
\end{equation*}
By taking logarithm to both sides and after some algebra,
\begin{equation*}
\begin{aligned}
&\log(1-p)-2\log (r+1)\\ &\simeq -\frac{\log Q_d (K,r)w_d (p,q)\log (K/r)}{\log
  (d-1)}+\log\log Q_d (K,r)\\ & \quad + \log c- \log r -\log\log
(d-1)\\ &\simeq -\log\log K - e\log r -1+ \log (1-q)^2 -\log\log (d-1)^2,\\
\end{aligned}
\end{equation*}
where we use $Q_d (K,r)=\log (K/r)/\log(d-1)$. Then
we have
\begin{equation*}
\begin{aligned}
\log r \simeq \log \left ( 1+\frac{2(1-p)\{1+(1-q)^2\}\log K}{e\log(d-1)}\right),
\end{aligned}
\end{equation*}
which implies that $r^{*}=\Theta\left(\frac{2(1-p)\{1+(1-q)^2\}\log K}{e\log(d-1)}\right)$ and this completes the proof.

\subsection{Deriving $r^*$ in \eqref{eqn:entropy3}}
For given $K,r$ and $d$, let
\begin{equation*}
\begin{aligned}
t_{d}(K,r,p,q)&:=  c\cdot e^{-(K/r)\log(K/r)} - \frac{Kh(p,q)+h(p,q)}{\frac{K (K/r)}{r}(\log (\frac{K}{2r}-1))},
\end{aligned}
\end{equation*}
where $h(p,q)= (1-H(p))+(1-p)(\log_2 d-H(q))$ and
$c=4d/3(d-2)$. Then one can check that
this is a differential unimodula function with respect to $r$.
We need to find $\frac{\partial t_{d}(K,r,p,q)}{\partial r}=0$ with respect to $r$ so that first consider
\begin{equation*}
\begin{aligned}
\frac{\partial \left(c\cdot e^{-(K/r)\log(K/r)}\right)}{\partial r}=\frac{cK\left(\frac{K}{r}\right)^{-K/r}r(\log (K/r)+1)}{r^2}.
\end{aligned}
\end{equation*}
Next, we also obtain that
\begin{equation*}
\begin{aligned}
\frac{\partial \left(\frac{Kh(p,q)+h(p,q)}{\frac{K (K/r)}{r}(\log (\frac{K}{2r}-1))}\right)}{\partial r}=\frac{(K+1)h(p,q)\left(\log(Kr/2)-2 \right)}{K(K/r)\left(\log(Kr/2)-1\right)^2}.
\end{aligned}
\end{equation*}
Let the above two equations are equal and after some algebra, we obtain
\begin{equation*}
\begin{aligned}
e^{\left(\frac{2(d-1)(r/7-1)}{7 dp(3H(p)+2dH(q))}\right)}&\simeq \log K.
\end{aligned}
\end{equation*}
By taking logarithm to both side then
\begin{equation*}
\begin{aligned}
r\simeq 1+\frac{7dp\{3H(p)+2dH(q)\}\log \log K}{2(d-1)}.
\end{aligned}
\end{equation*}
Therefore, we have $r^*= \left \lfloor 1+\frac{7 dp\{3H(p)+2dH(q)\}\log \log K}{2(d-1)}\right\rfloor$ for given $K$ and $q$ under $d$-regular tree and
completes the proof.

\subsection{Deriving $r^*$ in \eqref{eqn:detect2}}
For given $K,r$ and $d$, define
\begin{equation*}
\begin{aligned}
g_{d}&(K,r,p,q):= \\
& c (J_d (r,q))^3 \cdot \exp\left [-\left(p-\frac{1}{2}\right)^2\left(\frac{K}{r}\right)\log \left(\frac{K}{r}\right) \right],
\end{aligned}
\end{equation*}
where $J_d (r,q):= 1- e^{-\frac{r(d-1)(q-1/d)^2}{3d(1-q)}}$ and
$c=(8d+1)/d$. Then one can check that
this is a differential unimodula function with respect to $r$. Then,
by taking derivative $g_{d}(K,r,p,q)$ with respect to $r$ and by setting
$\frac{\partial g_{d}(K,r,p,q)}{\partial r}=0$, we have
\begin{equation*}
\begin{aligned}
&\frac{\partial g_{d}(K,r,p,q)}{\partial r}\\
&=\frac{\partial (c(J_{d}(r,q))^3)}{\partial r}\cdot \exp\left [-\left(p-\frac{1}{2}\right)^2\left(\frac{K}{r}\right)\log \left(\frac{K}{r}\right) \right]\\
&\qquad + c(J_{d}(r,q))^3\frac{\partial \left(e^{-2
    (p-1/2)^2 \left(\frac{K}{r}\right)\log
    \left(\frac{K}{r}\right)}\right)}{\partial r}=0.
\end{aligned}
\end{equation*}
Then, we first see that
\begin{equation*}
\begin{aligned}
\frac{\partial (c(J_{d}(r,q))^3)}{\partial r}&=\frac{c(d-1)(q-1/d)^2}{d(1-q)}\\
& \cdot e^{-\frac{r(d-1)(q-1/d)^2}{d(1-q)}}\left( e^{-\frac{r(d-1)(q-1/d)^2}{3d(1-q)}}-1\right)^2
\end{aligned}
\end{equation*}
Next, consider that
\begin{equation*}
\begin{aligned}
&\frac{\partial \left(e^{-2
    (p-1/2)^2 \left(\frac{K}{r}\right)\log
    \left(\frac{K}{r}\right)}\right)}{\partial r}=\\
  &\qquad\qquad\frac{K(1-2p)^2(K/r)^{-\frac{K(p-1/2)^2}{r}}(\log (K/r)+1)}{4r^2}.
\end{aligned}
\end{equation*}
Using these facts and after some algebra, we obtain
\begin{equation*}
\begin{aligned}
e^{\left(\frac{3(d-1)(r/7-1)}{2(1-p)^3 + (1-q)^2}\right)}&\simeq \log K.
\end{aligned}
\end{equation*}
By taking logarithm to both side then
\begin{equation*}
\begin{aligned}
r\simeq 1+\frac{7d^2 \{2(1-p)^3 + (1-q)^2\} \log\log
  K}{3(d-1)}.
\end{aligned}
\end{equation*}
Therefore, we have $r^*= \Theta \left(\frac{7d^2 \{2(1-p)^3 + (1-q)^2\} \log\log
  K}{3(d-1)}\right)$ for given $K$ and $q$ under $d$-regular tree and
completes the proof.

%
%
%
%
%%%% Local Variables:
%%%% mode: latex
%%%% TeX-master: "main"
%%%% End:
